# Supplementary material for: Optomechanical resource for fault-tolerant quantum computing
Source: arXiv:2505.00768 ancillary file (2025-07-08)
Supplement: Supplementary file 1 [file supp.pdf]

# Optomechanical resource for quantum computing: Supplementary

## CONTENTS

|                                                                                       |    |
|---------------------------------------------------------------------------------------|----|
| S1. Multimode optomechanics                                                           | 1  |
| A. Optical mode families                                                              | 4  |
| S2. Effective heating/cooling rates                                                   | 4  |
| A. Detailed balance                                                                   | 5  |
| B. System imperfections' effect on cooling                                            | 6  |
| S3. Quantum perspective on Bayes' theorem                                             | 6  |
| S4. Preparation of a single phonon/optomechanical two-mode squeezing                  | 7  |
| A. Evolution of expectation values                                                    | 7  |
| B. Two-mode squeezing as heating                                                      | 8  |
| C. Photons and phonons are generated in pairs                                         | 9  |
| D. Analytical calculation of heralding fidelity                                       | 9  |
| E. Heralding simulation                                                               | 10 |
| F. Heralded and anti-heralded phonon state                                            | 11 |
| S5. Retrieval of a single photon/optomechanical beam-splitting                        | 11 |
| A. Evolution of expectation values                                                    | 11 |
| B. Beam-splitting as cooling                                                          | 12 |
| S6. Minimum necessary OM coupling rate                                                | 12 |
| S7. Comparison of parallelized OM single-photon source to other single photon sources | 13 |
| S8. Error lifetimes of phononic dual-rail qubits                                      | 14 |
| S9. Single-shot GHZ-state preparation in phononic memories                            | 15 |
| A. GHZ-state heralding in an ideal system                                             | 16 |
| B. GHZ-state overlap with acoustic modes                                              | 17 |
| C. Probability of an arbitrary detection pattern with inefficient detectors           | 18 |
| D. "Herald-minus-one" detection probability                                           | 20 |
| E. Heralding simulations                                                              | 21 |
| S10. Iterative GHZ-state preparation in phononic memories (bleeding)                  | 21 |
| A. Bell state in 2 rounds                                                             | 23 |
| 1. Detection inefficiency and heralding fidelity                                      | 25 |
| B. Asymptotic success probabilities                                                   | 25 |
| C. Rounds-to-success with reset                                                       | 27 |
| 1. 2 qubits                                                                           | 27 |
| 2. 3 qubits                                                                           | 28 |
| S11. Other sources of entangled optical photons                                       | 30 |
| References                                                                            | 30 |

## S1. MULTIMODE OPTOMECHANICS

In this section, we sketch the derivation of the optomechanical Hamiltonian (Eq. (3) of the main text), following [1]. For this derivation, we include  $\hbar \neq 1$ . We start by considering the energy of an electromagnetic field in a non-magnetic

( $\mu = \mu_0$ ), dielectric medium:

$$H_{\text{EM}} = \frac{1}{2\mu_0} \int B^i(\mathbf{r})B^i(\mathbf{r}) d^3\mathbf{r} + \frac{1}{2\epsilon_0} \int D^i(\mathbf{r})\beta^{ij}(\mathbf{r})D^j(\mathbf{r}) d^3\mathbf{r}, \quad (\text{S1})$$

where  $\mathbf{B}$  is the magnetic field,  $\mathbf{D}$  is the electric displacement field, and  $\beta$  is the inverse relative dielectric tensor. The integral is taken over the entire resonator. Throughout this section, superscripts stand for Cartesian components and repeated indices are to be summed over. A table describing key values their units can be found at the end of this section. The optomechanical interaction arises from the influence of mechanical strain ( $S^{ij}(\mathbf{r})$ ) and displacement ( $\mathbf{u}(\mathbf{r})$ ) on the dielectric properties of a material. To quantify this effect, we decompose the inverse relative dielectric tensor into its background/reference value,  $\beta_{\text{ref}}$ , which is determined by the structure of the resonator, and the perturbation due to mechanical/acoustic deformations,  $\tilde{\beta}$ :

$$\beta(\mathbf{r}) = \beta_{\text{ref}}(\mathbf{r}) + \tilde{\beta}(\mathbf{r}; [\mathbf{u}(\mathbf{r})]). \quad (\text{S2})$$

Thus, the optomechanical Hamiltonian is

$$H_{\text{OM}} = \frac{1}{2\epsilon_0} \int \tilde{\beta}^{ij}(\mathbf{r}; [\mathbf{u}(\mathbf{r})])D^i(\mathbf{r})D^j(\mathbf{r}) d^3\mathbf{r}. \quad (\text{S3})$$

There are two main mechanisms for mechanical deformations to perturb dielectric properties: the photo-elastic effect via strain and the moving-boundary effect via displacement. Strain,  $S$ , and displacement,  $\mathbf{u}$ , are related by

$$S^{ij} = \frac{1}{2} \left( \frac{\partial u^i}{\partial r^j} + \frac{\partial u^j}{\partial r^i} \right). \quad (\text{S4})$$

The photoelastic contribution to the perturbation of the dielectric is

$$\tilde{\beta}_{\text{pe}}^{ij}(\mathbf{r}) = p^{ijkl}(\mathbf{r})S^{kl}(\mathbf{r}), \quad (\text{S5})$$

where  $p^{ijkl}(\mathbf{r})$  is the photoelastic tensor of the material at point  $\mathbf{r}$ . Acousto-optic coupling mediated by photoelasticity is typically dominant in systems whose size is much larger than the wavelength of light, and manifests throughout the volume of a dielectric medium, resulting in Brillouin scattering [2]. The moving-boundary effect is captured by

$$\tilde{\beta}_{\text{mb}}^{ij} = \beta_{\text{ref}}^{ij}(\mathbf{r} - \mathbf{u}(\mathbf{r})) - \beta_{\text{ref}}^{ij}(\mathbf{r}) \approx -\mathbf{u}(\mathbf{r}) \cdot (\nabla \beta_{\text{ref}}^{ij}(\mathbf{r})), \quad (\text{S6})$$

assuming the displacements are small relative to the size of the structure. The moving-boundary effect may also be understood as arising from radiation pressure. For systems with dimensions comparable to the wavelength of light, the moving-boundary effect can play a more significant role in the coupling [3].

In order to transform Eq. (S3) into the more familiar Hamiltonian terms of annihilation and creation operators, we decompose the optical and acoustic fields into their normal modes:

$$\mathbf{D}(\mathbf{r}, t) = \sum_{\alpha} \sqrt{\frac{\hbar\omega_{\alpha}}{2}} (\hat{a}_{\alpha}\mathbf{d}_{\alpha}(\mathbf{r})e^{-i\omega_{\alpha}t} + \text{h.c.}), \quad (\text{S7})$$

$$\mathbf{u}(\mathbf{r}, t) = \sum_{\lambda} \sqrt{\frac{\hbar\Omega_{\lambda}}{2}} (\hat{b}_{\lambda}\mathbf{u}_{\lambda}(\mathbf{r})e^{-i\Omega_{\lambda}t} + \text{h.c.}), \quad (\text{S8})$$

$$S(\mathbf{r}, t) = \sum_{\lambda} \sqrt{\frac{\hbar\Omega_{\lambda}}{2}} (\hat{b}_{\lambda}S_{\lambda}(\mathbf{r})e^{-i\Omega_{\lambda}t} + \text{h.c.}), \quad (\text{S9})$$

introducing the quantum annihilation operators  $\hat{a}_{\alpha}$  ( $\hat{b}_{\lambda}$ ) for optical (acoustic) modes, indexed by  $\alpha$  ( $\lambda$ ), and having frequencies  $\omega_{\alpha}$  ( $\Omega_{\lambda}$ ). This decomposition of the fields into modes relies on the assumption that the mode profiles do not change too much over their bandwidths. The optical and acoustic modes are discrete, rather than forming a band or continuum, because the system of interest is a resonator or cavity. The mode profiles  $\mathbf{d}_{\alpha}$ ,  $\mathbf{u}_{\lambda}$ , and  $S_{\lambda}$  are

determined by the structure of the system according to the wave equations

$$\nabla \times (\nabla \times \beta_{\text{ref}}(\mathbf{r}) \mathbf{d}_\alpha(\mathbf{r})) = \frac{\omega_\alpha^2}{c^2} \mathbf{d}_\alpha(\mathbf{r}) \quad (\text{S10})$$

$$\frac{\partial}{\partial r^j} c^{ijkl}(\mathbf{r}) S_\lambda^{kl}(\mathbf{r}) = -\Omega_\lambda^2 \rho(\mathbf{r}) u_\lambda^i(\mathbf{r}) \quad (\text{S11})$$

and the relationship between strain and displacement, Eq. (S4). Here,  $c^{ijkl}$  is the stiffness tensor and  $\rho$  is the mass density of the material. The mode profiles have normalizations

$$\frac{1}{\epsilon_0} \int \beta_{\text{ref}}^{ij}(\mathbf{r}) (d_\alpha^i(\mathbf{r}))^* d_\alpha^j(\mathbf{r}) d^3\mathbf{r} = 1, \quad (\text{S12})$$

$$\Omega_\lambda^2 \int \rho(\mathbf{r}) (u_\lambda^i(\mathbf{r}))^* u_\lambda^i(\mathbf{r}) d^3\mathbf{r} = 1, \quad (\text{S13})$$

$$\int c^{ijkl}(\mathbf{r}) (S_\lambda^{ij}(\mathbf{r}))^* S_\lambda^{kl}(\mathbf{r}) d^3\mathbf{r} = 1. \quad (\text{S14})$$

With these definitions, the non-interacting part of the resonator Hamiltonian is

$$H_0 = \sum_\alpha \hbar \omega_\alpha \hat{a}_\alpha^\dagger \hat{a}_\alpha + \sum_\lambda \hbar \Omega_\lambda \hat{b}_\lambda^\dagger \hat{b}_\lambda, \quad (\text{S15})$$

neglecting zero-point energy.

We determine the photo-elastic contribution to the interaction Hamiltonian by substituting Eqs. (S7) and (S9) into (S5) and then (S3).

$$H_{\text{OM,pe}} = \frac{1}{2\epsilon_0} \sum_\lambda \sum_{\alpha,\gamma} \sqrt{\frac{\hbar \Omega_\lambda}{2}} \sqrt{\frac{\hbar \omega_\alpha}{2}} \sqrt{\frac{\hbar \omega_\gamma}{2}} \int p^{ijkl} \left( \hat{b}_\lambda S_\lambda^{kl} e^{-i\Omega_\lambda t} + \text{h.c.} \right) \left( \hat{a}_\alpha d_\alpha^i e^{-i\omega_\alpha t} + \text{h.c.} \right) \left( \hat{a}_\gamma d_\gamma^j e^{-i\omega_\gamma t} + \text{h.c.} \right) d^3\mathbf{r}. \quad (\text{S16})$$

In this and future expressions, the first sum is taken over all acoustic modes of the resonator, which are indexed by  $\lambda$ . The second sum is a double sum over the optical modes, indexed by  $\alpha$  and  $\gamma$ . We perform the same substitutions for moving-boundary contribution (Eqs. (S8) and (S6)), and obtain the generic Hamiltonian

$$H_{\text{OM}} = \hbar \sum_\lambda \sum_{\alpha,\gamma} \left[ g_{\lambda\alpha\gamma} \hat{b}_\lambda \hat{a}_\alpha \hat{a}_\gamma^\dagger e^{-i(\Omega_\lambda + \omega_\alpha - \omega_\gamma)t} + \text{h.c.} \right], \quad (\text{S17})$$

where

$$g_{\lambda\alpha\gamma} = \frac{1}{\hbar \epsilon_0} \sqrt{\frac{\hbar \Omega_\lambda}{2}} \sqrt{\frac{\hbar \omega_\alpha}{2}} \sqrt{\frac{\hbar \omega_\gamma}{2}} \int d_\alpha^i(\mathbf{r}) (d_\gamma^j(\mathbf{r}))^* \left( p^{ijkl}(\mathbf{r}) S_\lambda^{kl}(\mathbf{r}) - \mathbf{u}_\lambda(\mathbf{r}) \cdot \nabla \beta_{\text{ref}}^{ij}(\mathbf{r}) \right) d^3\mathbf{r} \quad (\text{S18})$$

is the total coupling rate between acoustic mode  $\lambda$  and optical modes  $\alpha$  and  $\gamma$ . We have taken the rotating wave approximation in Eq. (S17) to drop terms which create or destroy two photons because  $\omega_\alpha \sim 200$  THz. We have dropped terms arising from quantum vacuum fluctuations because they will not meaningfully affect the behavior given a classical drive. Exactly which terms in Eq. (S17) are appreciable will depend on the magnitudes of the various  $g_{\lambda\alpha\gamma}$  and how strictly the energy conservation condition  $\omega_\alpha - \omega_\gamma + \Omega_\lambda = 0$  needs to be satisfied. The coupling rates  $g_{\lambda\alpha\gamma}$  depend on mode overlap and phase matching, i.e. symmetry and momentum conservation, as well as material properties.

The coupling rates from the main text are  $g_0 = g_{0\text{r}0}$  and  $g_h = g_{0\text{h}b}$  using the notation of Eq. (S18) and assigning the sole acoustic mode index 0. It is common for  $g_{\lambda\alpha\gamma}$  and  $g_{\lambda\gamma\alpha}$  to be very different in extended systems. This allows the studied interaction Hamiltonian, Eq. (3), to exclude terms such as  $\hat{a}_0 \hat{a}_i^\dagger \hat{b}$  before taking the rotating-wave approximation. We have also assumed that the various  $g_{0\alpha\alpha}$ , which describe conventional cavity optomechanical interactions, are small.

| Symbol       | Meaning                            | Units                           |
|--------------|------------------------------------|---------------------------------|
| $\epsilon_0$ | Vacuum permittivity                | $\text{F} \cdot \text{m}^{-1}$  |
| $\beta$      | Inverse relative dielectric tensor | 1                               |
| $\mathbf{D}$ | Electric displacement field        | $\text{C} \cdot \text{m}^{-2}$  |
| $\mathbf{u}$ | Displacement                       | m                               |
| $S^{ij}$     | Strain                             | 1                               |
| $\rho$       | Mass density                       | $\text{kg} \cdot \text{m}^{-3}$ |
| $c^{ijkl}$   | Stiffness tensor                   | $\text{N} \cdot \text{m}^{-2}$  |
| $p^{ijkl}$   | Photoelastic tensor                | 1                               |

### A. Optical mode families

The total optical field in the resonator is given by Eq. (S7). In many systems, the mode profiles may be decomposed into a transverse and longitudinal components, and the polarization is constant:  $\mathbf{d}_\alpha(\mathbf{r}) = d_{\alpha,\perp}(x, y)d_{\alpha,\parallel}(z)\mathbf{e}_\alpha$ . An optical mode family is a set of modes which all have the same (or almost same) transverse mode profile and polarization.

## S2. EFFECTIVE HEATING/COOLING RATES

If optical decay is the fastest rate in the system, the optomechanical interaction can be modeled as an effective heating or cooling of the acoustic mode. We neglect other forms of acoustic loss for the time being. Following [4], we consider an undamped system  $S$  which is coupled to a reservoir  $R$ . Generically,

$$H = H_S + H_R + H_{SR}. \quad (\text{S19})$$

Here, the “system” is the acoustic mode:

$$H_S \rightarrow \Omega \hat{b}^\dagger \hat{b}, \quad (\text{S20})$$

the “reservoir” is the optical modes:

$$H_R \rightarrow \omega_1 \hat{a}_1^\dagger \hat{a}_1 + \omega_2 \hat{a}_2^\dagger \hat{a}_2, \quad (\text{S21})$$

and the interaction is the optomechanical interaction:

$$H_{SR} = (\hat{b}\hat{\Lambda}^\dagger + \hat{b}^\dagger\hat{\Lambda}) \rightarrow H_{\text{OM}} = g(\hat{b}\hat{a}_1\hat{a}_2^\dagger + \hat{b}^\dagger\hat{a}_1^\dagger\hat{a}_2). \quad (\text{S22})$$

We treat the optical modes as memoryless reservoirs which are unaffected by their interaction with the acoustic mode (Born approximation). With this assumption, the evolution of the acoustic mode state is

$$\begin{aligned} \dot{\tilde{\rho}}(t) = - \int_0^t d\tau \left\{ \left[ \hat{b}\hat{b}^\dagger \tilde{\rho}(t-\tau) - \hat{b}^\dagger \tilde{\rho}(t-\tau) \hat{b} \right] e^{-i\Omega\tau} \langle \tilde{\Lambda}^\dagger(t) \tilde{\Lambda}(t-\tau) \rangle_R + \text{h.c.} \right. \\ \left. + \left[ \hat{b}^\dagger \tilde{\rho}(t-\tau) - \tilde{\rho}(t-\tau) \hat{b}^\dagger \right] e^{i\Omega\tau} \langle \tilde{\Lambda}(t) \tilde{\Lambda}^\dagger(t-\tau) \rangle_R + \text{h.c.} \right\}, \quad (\text{S23}) \end{aligned}$$

where  $\tilde{\rho}(t)$  is the density matrix of the acoustic mode (i.e. with the optical reservoir traced out) in the rotating frame of the uncoupled system and reservoir Hamiltonians, and  $\tilde{\Lambda}(t)$  is the reservoir operator which mediates the system-reservoir interaction, also in the rotating frame:  $\tilde{\Lambda}(t) = g\hat{a}_1^\dagger\hat{a}_2 e^{i(\omega_1 - \omega_2)t}$ . The subscript in  $\langle \rangle_R$  indicates that the expectation value is taken only with respect to the reservoir.

If  $\hat{a}_1$ , but not  $\hat{a}_2$ , is driven (cooling), the reservoir expectation values are

$$\langle \tilde{\Lambda}(t) \tilde{\Lambda}^\dagger(t - \tau) \rangle_R = |g\alpha_1|^2 e^{-i(\omega_2 - \omega_1)\tau} e^{-\kappa_2 \tau/2} \quad (\text{S24})$$

$$\langle \tilde{\Lambda}^\dagger(t) \tilde{\Lambda}(t - \tau) \rangle_R = 0, \quad (\text{S25})$$

where  $\alpha_1$  is the steady-state amplitude in mode  $\hat{a}_1$  and  $\kappa_2$  is the decay rate of mode  $\hat{a}_2$ . If  $\hat{a}_2$ , but not  $\hat{a}_1$ , is driven (heating), the reservoir expectation values are

$$\langle \tilde{\Lambda}(t) \tilde{\Lambda}^\dagger(t - \tau) \rangle_R = 0 \quad (\text{S26})$$

$$\langle \tilde{\Lambda}^\dagger(t) \tilde{\Lambda}(t - \tau) \rangle_R = |g\alpha_2|^2 e^{i(\omega_2 - \omega_1)\tau} e^{-\kappa_1 \tau/2}, \quad (\text{S27})$$

where  $\alpha_2$  is the steady-state amplitude in mode  $\hat{a}_2$  and  $\kappa_1$  is the decay rate of mode  $\hat{a}_1$ . Returning to the case of cooling, substituting Eqs. (S24)–(S25) into Eq. (S23) yields

$$\dot{\tilde{\rho}}(t) = - \int_0^t d\tau \left\{ \left[ \hat{b}^\dagger \hat{b} \tilde{\rho}(t - \tau) - \tilde{\rho}(t - \tau) \hat{b}^\dagger \right] |g\alpha_1|^2 e^{-i(\omega_2 - \omega_1 - \Omega)\tau} e^{-\kappa_2 \tau/2} + \text{h.c.} \right\}. \quad (\text{S28})$$

If  $e^{-i(\omega_2 - \omega_1 - \Omega)\tau} e^{-\kappa_2 \tau/2}$  is strongly peaked around  $\tau = 0$  and  $\tilde{\rho}(t)$  doesn't vary too quickly, i.e. if  $\kappa_2 \gg |g\alpha_1|$ , we may take the Markov approximation,  $\tilde{\rho}(t - \tau) \approx \tilde{\rho}(t)$ , and extend the upper limit of the integral to  $\infty$ . This yields the equation of motion for the density matrix in the interaction frame  $\dot{\tilde{\rho}} = \Gamma_{\text{opt}}^\downarrow \mathcal{D}[\hat{b}] \tilde{\rho}$ , where the effective, optically-induced cooling rate is

$$\Gamma_{\text{opt}}^\downarrow = \frac{\kappa_2 |g\alpha_1|^2}{(\kappa_2/2)^2 + (\omega_2 - \omega_1 - \Omega)^2}, \quad (\text{S29})$$

and we have introduced the dissipation super-operator

$$\mathcal{D}[\hat{b}] \hat{\rho} = \hat{b} \hat{\rho} \hat{b}^\dagger - \frac{1}{2} (\hat{b}^\dagger \hat{b} \hat{\rho} + \hat{\rho} \hat{b}^\dagger \hat{b}). \quad (\text{S30})$$

If, on the other hand, optical mode  $\hat{a}_2$  is driven, the evolution of the density matrix follows  $\dot{\tilde{\rho}} = \Gamma_{\text{opt}}^\uparrow \mathcal{D}[\hat{b}^\dagger] \tilde{\rho}$ , where the effective, optically-induced heating rate is

$$\Gamma_{\text{opt}}^\uparrow = \frac{\kappa_1 |g\alpha_2|^2}{(\kappa_1/2)^2 + (\omega_2 - \omega_1 - \Omega)^2}. \quad (\text{S31})$$

### A. Detailed balance

In addition to effective heating and cooling from the optomechanical interaction, the acoustic mode also undergoes thermal cooling (rate  $\Gamma_{\text{th}}^\downarrow = \Gamma(n_{\text{th}} + 1)$ ) and heating (rate  $\Gamma_{\text{th}}^\uparrow = \Gamma n_{\text{th}}$ ), where  $n_{\text{th}}$  is the phonon population at thermal equilibrium (no external drives). Loss and gain rates may be simply added to find the steady state population in the acoustic mode. Given total loss rate  $\Gamma_{\text{tot}}^\downarrow$  and total gain rate  $\Gamma_{\text{tot}}^\uparrow$ , the phonon population ( $n_{\text{ph}} = \langle \hat{b}^\dagger \hat{b} \rangle$ ) changes according to  $\dot{n}_{\text{ph}} = -\Gamma_{\text{tot}}^\downarrow n_{\text{ph}} + \Gamma_{\text{tot}}^\uparrow (n_{\text{ph}} + 1)$ . The steady state phonon population is

$$n_{\text{ph}} \rightarrow \frac{1}{\Gamma_{\text{tot}}^\downarrow / \Gamma_{\text{tot}}^\uparrow - 1}. \quad (\text{S32})$$

A steady state only exists if  $\Gamma_{\text{tot}}^\downarrow > \Gamma_{\text{tot}}^\uparrow$ .<sup>1</sup> Combining Eq. (S32) with (S31) and (S29) gives the cooled population Eq. (7), reproduced here:

$$n_{\text{ph}} \rightarrow \frac{n_{\text{th}}}{(C_0 |\alpha_r|^2 + 1)}.$$

---

<sup>1</sup> This is an artifact of neglecting pump depletion, which would limit the growth of the phonon population if  $\Gamma_{\text{tot}}^\uparrow > \Gamma_{\text{tot}}^\downarrow$

### B. System imperfections' effect on cooling

In practice, the resonator may support optomechanical interactions beyond the desired ones. In this section, we calculate how those interactions may limit the cooling performance of the resonator. We consider three possible interactions when the red mode,  $\hat{a}_r$ , is driven: (1) the desired interaction between the acoustic mode  $\hat{b}$  and the output mode  $\hat{a}_0$ , which cools the acoustic mode, (2) a potential interaction between  $\hat{b}$  and an undesired optical Stokes mode  $\hat{a}_S$ , which heats the acoustic mode, and (3) a potential interaction between  $\hat{b}$  and scattering within the driven red mode  $\hat{a}_r$ , which both heats and cools the acoustic mode. Therefore, the total cooling rate is

$$\Gamma_{\text{tot}}^{\downarrow} = \underbrace{(g_0^2 \kappa_0 |\chi_0(\Omega)|^2)}_{(1)} + \underbrace{(g_r^2 \kappa_r |\chi_r(0)|^2)}_{(3)} n_r + \underbrace{\Gamma(n_{\text{th}} + 1)}_{\text{thermal}}, \quad (\text{S33})$$

and the total heating rate is

$$\Gamma_{\text{tot}}^{\uparrow} = \underbrace{(g_S^2 \kappa_S |\chi_S(\omega_r - \omega_S)|^2)}_{(2)} + \underbrace{(g_r^2 \kappa_r |\chi_r(0)|^2)}_{(3)} n_r + \underbrace{\Gamma n_{\text{th}}}_{\text{thermal}}, \quad (\text{S34})$$

where  $|\chi_i(\omega)|^2 = ((\omega - \Omega)^2 + (\kappa_i/2)^2)^{-1}$  are the response functions for each optomechanical process,  $g_i$  are their respective coupling rates, and  $n_r$  is the population of the driven optical mode. The first term in Eq. (S33) (Eq. (S34)) is Eq. (S29) (Eq. (S31)) with mode assignments  $1 \rightarrow 0$  and  $2 \rightarrow r$  ( $1 \rightarrow r$  and  $2 \rightarrow S$ ). The heating and cooling rates for the intramodal process (the second term in each of Eq. (S33)–(S34)) are derived in [5].

From here, in conjunction with Eq. (S32), we can find the phonon population in high pump power limit ( $n_r \rightarrow \infty$ ):

$$n_{\text{ph}} \rightarrow \frac{g_r^2 \kappa_r |\chi_r(0)|^2 + g_S^2 \kappa_S |\chi_S(\omega_r - \omega_S)|^2}{g_0^2 \kappa_0 |\chi_0(\Omega)|^2 - g_S^2 \kappa_S |\chi_S(\omega_r - \omega_S)|^2}. \quad (\text{S35})$$

Notice that, unlike the ideal case Eq. (7), there is a floor on how far we can cool the acoustic mode determined by the optical mode structure and coupling rates.

### S3. QUANTUM PERSPECTIVE ON BAYES' THEOREM

We show that it is valid to use Bayes' theorem in a quantum context to calculate heralding fidelity, as we do in Sec. IIB and IIIB1 of the main text. We consider a system with optical loss and/or noise but not acoustic loss (Fig. S1). The acoustic and optical subsystems are initially separable and are entangled by a lossless interaction  $\hat{U}_{ab}$ . The operator  $\hat{U}_{ab}$  includes any unitary transformations on the individual subsystems. The optical subsystem is subjected to a lossy/noisy quantum channel  $\mathcal{E}_a$ . The optical subsystem is measured destructively, which we represent as the optical subsystem being projected onto state  $|\phi\rangle_a$  and traced out. This leaves the acoustic modes in the state  $\rho_{b|\text{h}}$ . The heralding fidelity is the square overlap between the actual heralded state,  $\rho_{b|\text{h}}$ , and the ideal or expected state,  $|\psi_{\text{h}}\rangle_b$ .

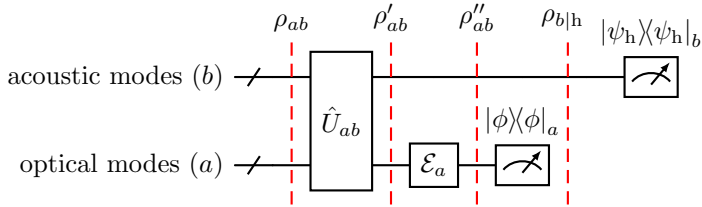

FIG. S1. **Model for demonstrating validity of Bayes' theorem in quantum systems.** Upper and lower wires represent bundles of acoustic (b) and optical (a) modes, respectively.

All together, the process is

$$\rho_{ab} = \rho_a \otimes \rho_b \rightarrow \rho'_{ab} = \hat{U}_{ab} \rho_{ab} \hat{U}_{ab}^{\dagger} \rightarrow \rho''_{ab} = \mathcal{E}_a(\rho'_{ab}) \rightarrow \rho_{b|\text{h}} = \frac{\text{Tr}_a\{|\phi\rangle\langle\phi|_a \rho''_{ab}\}}{\text{Tr}_{ab}\{|\phi\rangle\langle\phi|_a \rho''_{ab}\}} \quad (\text{S36})$$

where  $\text{Tr}_a\{\bullet\}$  is the partial trace over the optical modes<sup>2</sup> and  $\text{Tr}_{ab}\{\bullet\}$  is the full trace. We omit subsystem identity operators, e.g.  $|\phi\rangle\langle\phi|_a = |\phi\rangle\langle\phi|_a \otimes \hat{I}_b$ . Therefore, the heralding fidelity is

$$\begin{aligned} F_h &:= \langle \psi_h |_b \rho_{b|h} | \psi_h \rangle_b = \frac{\text{Tr}_b \{ |\psi_h\rangle\langle\psi_h|_b \text{Tr}_a \{ |\phi\rangle\langle\phi|_a \rho''_{ab} \} \}}{\text{Tr}_{ab} \{ |\phi\rangle\langle\phi|_a \rho''_{ab} \}} \\ &= \frac{\text{Tr}_{ab} \{ |\psi_h\rangle\langle\psi_h|_b |\phi\rangle\langle\phi|_a \mathcal{E}_a(\rho'_{ab}) \}}{\text{Tr}_{ab} \{ |\phi\rangle\langle\phi|_a \rho''_{ab} \}} \\ &= \frac{\text{Tr}_a \{ |\phi\rangle\langle\phi|_a \mathcal{E}_a(\text{Tr}_b \{ |\psi_h\rangle\langle\psi_h|_b \rho'_{ab} \}) \}}{\text{Tr}_{ab} \{ |\phi\rangle\langle\phi|_a \rho''_{ab} \}}, \end{aligned} \quad (\text{S37})$$

where  $\text{Tr}_b\{\bullet\}$  is the partial trace over the acoustic modes.<sup>3</sup> For the final equality, we used the associativity of partial traces and the fact that the loss operator  $\mathcal{E}_a$  acts only on the optical subsystem.

Bayes' theorem states

$$P(\text{A.S. in } |\psi_h\rangle_b \mid \text{O.S. meas. in } |\phi\rangle_a) = \frac{P(\text{O.S. meas. in } |\phi\rangle_a \mid \text{A.S. in } |\psi_h\rangle_b) P(\text{A.S. in } |\psi_h\rangle_b)}{P(\text{O.S. meas. in } |\phi\rangle_a)}, \quad (\text{S38})$$

where A.S. stands for ‘‘acoustic subsystem,’’ O.S. stands for ‘‘optical subsystem,’’ meas. stands for ‘‘measured,’’ and  $P(x|y)$  is the conditional probability of  $x$  given  $y$ . The correspondences between the quantum expression (Eq. (S37)) and Bayes' theorem (Eq. (S38)) are

$$\begin{aligned} P(\text{A.S. in } |\psi_h\rangle_b \mid \text{O.S. meas. in } |\phi\rangle_a) &\Leftrightarrow F_h = \langle \psi_h |_b \rho_{b|h} | \psi_h \rangle_b, \\ P(\text{O.S. meas. in } |\phi\rangle_a \mid \text{A.S. in } |\psi_h\rangle_b) &\Leftrightarrow \text{Tr}_a \left\{ |\phi\rangle\langle\phi|_a \mathcal{E}_a \left( \frac{\text{Tr}_b \{ |\psi_h\rangle\langle\psi_h|_b \rho'_{ab} \}}{\text{Tr}_{ab} \{ |\psi_h\rangle\langle\psi_h|_b \rho'_{ab} \}} \right) \right\}, \\ P(\text{A.S. in } |\psi_h\rangle_b) &\Leftrightarrow \text{Tr}_{ab} \{ |\psi_h\rangle\langle\psi_h|_b \rho'_{ab} \} = \text{Tr}_{ab} \{ |\psi_h\rangle\langle\psi_h|_b \rho''_{ab} \}, \\ P(\text{O.S. meas. in } |\phi\rangle_a) &\Leftrightarrow \text{Tr}_{ab} \{ |\phi\rangle\langle\phi|_a \rho''_{ab} \}. \end{aligned}$$

## S4. PREPARATION OF A SINGLE PHONON/OPTOMECHANICAL TWO-MODE SQUEEZING

### A. Evolution of expectation values

In this section, we describe how the OM system evolves under two-mode squeezing and show that the number of photon-phonon pairs follows a thermal distribution. The Hamiltonian of interest is Eq. (5), reproduced here:

$$\hat{H}_{\text{sq}} = g_h(\alpha_b \hat{a}_h^\dagger \hat{b}^\dagger + \alpha_b^* \hat{a}_h \hat{b}).$$

Pump depletion is negligible because  $g_h^2 \langle \hat{a}_h^\dagger \hat{a}_h \hat{b}^\dagger \hat{b} \rangle \ll (\kappa_b/2)^2 |\alpha_b|^2$ . We assume both modes start in vacuum.

If we neglect all losses,  $\hat{H}_{\text{sq}}$  generates the photon-phonon squeezed state

$$|\psi(t)\rangle = \sqrt{p_0} \sum_n (-i)^n (1 - p_0)^{n/2} |n, n\rangle, \quad (\text{S39})$$

where  $p_0 = \text{sech}^2(g_h |\alpha_b| t)$  is the probability of having no photon-phonon pairs. The right-hand side of Eq. (S39) is written in the joint number basis: the first index in the ket is the number of herald photons and the second index is the number of phonons. The coefficients describe a geometric distribution. If either mode is traced out, the remaining mode is in a thermal state. The expected populations are  $\langle \hat{a}_h^\dagger \hat{a}_h \rangle = \langle \hat{b}^\dagger \hat{b} \rangle = \sinh^2(g_h |\alpha_b| t)$ .

We now incorporate optical loss while continuing to neglect acoustic loss. The equations of motion for the expected

<sup>2</sup>  $\text{Tr}_a\{\rho\}$  is the full trace if  $\rho$  only includes optical modes (i.e. if acoustic modes have already been traced out).

<sup>3</sup>  $\text{Tr}_b\{\rho\}$  is the full trace if  $\rho$  only includes acoustic modes (i.e. if optical modes have already been traced out).

numbers of excitations in the regime are

$$\dot{n}_a = g\sigma - \kappa n_a, \quad (\text{S40})$$

$$\dot{n}_{\text{ph}} = g\sigma, \quad (\text{S41})$$

$$\dot{\sigma} = 2g(n_a + n_{\text{ph}} + 1) - \frac{\kappa}{2}\sigma, \quad (\text{S42})$$

where  $n_a = \langle \hat{a}_{\text{h}}^\dagger \hat{a}_{\text{h}} \rangle$  is the herald-photon population,  $n_{\text{ph}} = \langle \hat{b}^\dagger \hat{b} \rangle$  is the phonon population,  $\sigma = i\langle \hat{a}_{\text{h}} \hat{b} - \hat{a}_{\text{h}}^\dagger \hat{b}^\dagger \rangle$ , and  $g = g_{\text{h}}\alpha_{\text{b}}$ . We have let  $\alpha_{\text{b}} = |\alpha_{\text{b}}|$ . If  $g$  is constant (continuous driving), these equations of motions are satisfied by

$$n_a = (g/\tilde{g})^2 e^{-\kappa t/2} \sinh^2(\tilde{g}t), \quad (\text{S43})$$

$$n_{\text{ph}} = e^{-\kappa t/2} \left( \cosh(\tilde{g}t) + \frac{\kappa}{4\tilde{g}} \sinh(\tilde{g}t) \right)^2 - 1, \quad (\text{S44})$$

$$\sigma = 2(g/\tilde{g})e^{-\kappa t/2} \sinh(\tilde{g}t) \left( \cosh(\tilde{g}t) + \frac{\kappa}{4\tilde{g}} \sinh(\tilde{g}t) \right) \quad (\text{S45})$$

where  $\tilde{g} = \sqrt{(g_{\text{h}}\alpha_{\text{b}})^2 + (\kappa_{\text{h}}/4)^2}$  is the effective coupling rate. Eq. (S44) is the same as Eq. (8).

To investigate the statistics of the photons and phonons, we find equations of motion for higher-order expectation values:

$$\dot{q}_a = 2gy_a - 2\kappa q_a \quad \dot{y}_a = g(4(n_2 + n_a) + 2q_a - s_2) - \frac{3\kappa}{2}y_a \quad (\text{S46})$$

$$\dot{q}_b = 2gy_b \quad \dot{y}_b = g(4(n_2 + n_{\text{ph}}) + 2q_b - s_2) - \frac{\kappa}{2}y_b \quad (\text{S47})$$

$$\dot{s}_2 = -2g(y_a + y_b + 2\sigma) - \kappa s_2 \quad \dot{n}_2 = g(y_a + y_b + \sigma) - \kappa n_2, \quad (\text{S48})$$

where

$$q_a = \langle (\hat{a}_{\text{h}}^\dagger)^2 \hat{a}_{\text{h}}^2 \rangle \quad y_a = i \langle (\hat{a}_{\text{h}}^\dagger \hat{a}_{\text{h}})(\hat{a}_{\text{h}} \hat{b}) - (\hat{a}_{\text{h}}^\dagger \hat{b}^\dagger)(\hat{a}_{\text{h}}^\dagger \hat{a}_{\text{h}}) \rangle \quad (\text{S49})$$

$$q_b = \langle (\hat{b}^\dagger)^2 \hat{b}^2 \rangle \quad y_b = i \langle (\hat{b}^\dagger \hat{b})(\hat{a}_{\text{h}} \hat{b}) - (\hat{a}_{\text{h}}^\dagger \hat{b}^\dagger)(\hat{b}^\dagger \hat{b}) \rangle \quad (\text{S50})$$

$$s_2 = \langle \hat{a}_{\text{h}}^2 \hat{b}^2 \rangle + \langle (\hat{a}_{\text{h}}^\dagger)^2 (\hat{b}^\dagger)^2 \rangle \quad n_2 = \langle \hat{a}_{\text{h}}^\dagger \hat{a}_{\text{h}} \hat{b}^\dagger \hat{b} \rangle. \quad (\text{S51})$$

This set of equations be transformed into a pair of coupled second-order differential equations involving only  $y_{\text{tot}} = y_a + y_b$ ,  $\Delta q = q_a - q_b$ , and lower-order expectation values,  $n_a$ ,  $n_{\text{ph}}$ , and  $\sigma$ . The solution to this pair of equations then can be used to find expressions for (S49)–(S51). These expressions give  $q_a = 2n_a^2$  and  $q_b = 2n_{\text{ph}}^2$ , which can be transformed into  $\text{var}(n_a) = n_a(n_a + 1)$  and  $\text{var}(n_{\text{ph}}) = n_{\text{ph}}(n_{\text{ph}} + 1)$ , suggesting that the photon and phonon numbers each follow thermal statistics even in the presence of loss.

## B. Two-mode squeezing as heating

The fastest-growing term in Eq. (S44) for the phonon population has rate

$$\Gamma_{\text{eff}}^\uparrow = 2\tilde{g}_{\text{h}} - \frac{\kappa_{\text{h}}}{2} \approx \frac{4|g\alpha_{\text{b}}|^2}{\kappa_{\text{h}}} = \Gamma_{\text{opt}}^\uparrow. \quad (\text{S52})$$

The approximation requires  $16|g\alpha_{\text{b}}|^2 \ll \kappa_{\text{h}}^2$ . This shows the validity of the effective heating rate formulation, Eq. (S31) for moderate drive strength.

### C. Photons and phonons are generated in pairs

$\hat{H}_{\text{sq}}$  generates photon-phonon pairs. That is, the *cumulative* number of phonons and photons generated are equal. We define the time-dependent cumulative number operators for the acoustic mode and the optical herald mode as

$$\hat{N}_{\text{ph}}(t) := \hat{n}_{\text{ph}}(t) + \Gamma \int_0^t \hat{n}_{\text{ph}}(t') dt', \quad (\text{S53})$$

$$\hat{N}_a(t) := \hat{n}_a(t) + \kappa_h \int_0^t \hat{n}_a(t') dt', \quad (\text{S54})$$

respectively. Here,  $\hat{n}_{\text{ph}}(t)$  and  $\hat{n}_a(t)$  are the instantaneous resonator population operators for the phonons and the herald photons, respectively, in the Heisenberg picture.<sup>4</sup> The time-integral terms, e.g.  $\kappa_h \int_0^t \hat{n}_a(t') dt'$ , count the particles which have left the resonator between time 0 and time  $t$ . The cumulative number operators evolve according to

$$\frac{d\hat{N}_{\text{ph}}}{dt} = \frac{d\hat{n}_{\text{ph}}}{dt} + \Gamma \hat{n}_{\text{ph}}, \quad (\text{S55})$$

etc. If the only interaction is two-mode squeezing, the instantaneous number operators evolve as

$$\frac{d\hat{n}_{\text{ph}}}{dt} = ig_h \alpha_b (\hat{a}_h \hat{b} - \hat{a}_h^\dagger \hat{b}^\dagger) - \Gamma \hat{n}_{\text{ph}}, \quad (\text{S56})$$

etc., assuming  $\alpha_b = |\alpha_b|$ . Therefore,  $\frac{d\hat{N}_a}{dt} = \frac{d\hat{N}_{\text{ph}}}{dt}$ . Because both modes to start in vacuum, we have  $\langle \hat{N}_{\text{ph}}^k \rangle = \langle \hat{N}_a^k \rangle$  for all  $k$  and  $t > 0$ . This allows us to say that the cumulative number distributions for the photon and phonon are equal, i.e. that the photons and phonons are generated in pairs. This is stronger than simply saying that the cumulative numbers of photons and phonons are equal in expectation.

### D. Analytical calculation of heralding fidelity

In this section, we give the full expressions for the single-phonon heralding probability and fidelity (Sec. II B). The heralding fidelity is calculated from the Bayesian expression, Eq. (9), reproduced here:

$$F_{\text{h,sp}} = P(\text{single phonon}|\text{herald}) = P(\text{herald}|\text{single phonon}) \frac{P(\text{single phonon})}{P(\text{herald})}. \quad (\text{S57})$$

We continue to neglect acoustic loss because the duration of the squeezing interaction is much shorter than the phonon lifetime.

The total herald probability  $P(\text{herald})$  includes every possible way the detector could register one single photon. If more than 1 photon-phonon pair is generated, there is a herald if the detector detects one photon and misses all others. Even if no photon-phonon pairs are produced, the detector may produce, with probability  $p_d$ , a dark count due to thermal or shot noise.<sup>5</sup> Accounting for all possibilities,

$$P(\text{herald}) = p_d p_0 + \sum_{k=1}^{\infty} \binom{k}{1} \eta (1-\eta)^{k-1} p_0 (p_1/p_0)^k. \quad (\text{S58})$$

The term inside the summation is the product of the probability of a herald given  $k$  photon-phonon pairs and the probability of producing  $k$  photon-phonon pairs.  $\binom{k}{1} = k$  is a binomial coefficient. The approximate expression Eq. (10) includes only the first two terms in the infinite sum. Evaluating the full sum yields

$$p_{\text{h,sp}} := P(\text{herald}) = \frac{\eta p_1}{(1 - (p_1/p_0)(1-\eta))^2} + p_d p_0. \quad (\text{S59})$$

<sup>4</sup> The Heisenberg-picture operators may not be decomposed, i.e.  $\hat{n}_{\text{ph}}(t) \neq \hat{b}^\dagger(t)\hat{b}(t)$  and  $\hat{n}_a(t) \neq \hat{a}_h^\dagger(t)\hat{a}_h(t)$ , because the time evolution includes loss and is non-unitary.

<sup>5</sup> The possibility that photon-phonon pairs were generated, all photons fail to be detected, and there is a dark count is negligible.

All together, the heralding fidelity is

$$F_{h,sp} = \left( \frac{1}{(1 - (p_1/p_0)(1 - \eta))^2} + \frac{p_d p_0}{\eta p_1} \right)^{-1}. \quad (\text{S60})$$

The operating regime has  $p_d \ll p_1 \ll 1$ . Therefore, we first approximate  $1 - F_{h,sp}$  to first order in  $p_d$ , then to first order in  $p_1$ , and finally drop terms proportional to  $p_d$  but not  $1/p_1$ . This gives Eq. (11).

### E. Heralding simulation

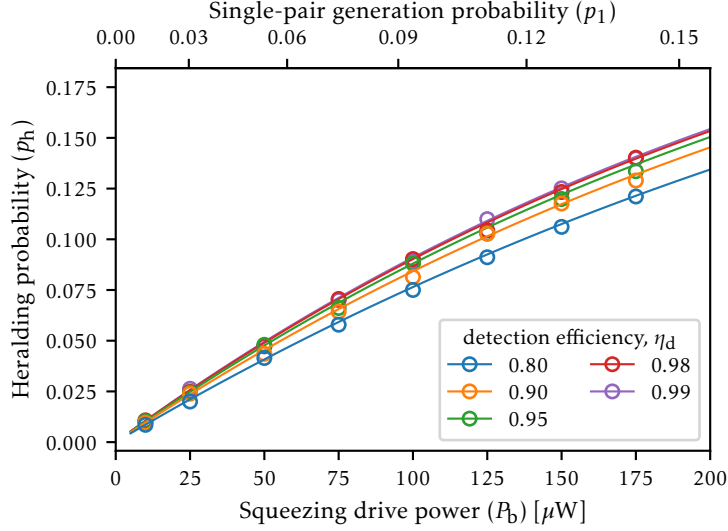

FIG. S2. Dependence of heralding probability on peak squeezing drive power. Secondary  $x$  axis shows  $p_1$ , the single photon-phonon pair generation probability, whose dependence on drive power is sublinear. Lines show semi-analytical results. Each dot represents the average result of 50,000 stochastic QuTiP simulations [6–8]. Detector dark counts are not included in this simulation.

The heralding process is simulated using the `photocurrent_mesolve` function of QuTiP v4.7 [6–8]. This stochastic simulation outputs a photodetector trace and the density matrix over time. The simulation considers “deterministic” and “stochastic” collapse operators separately. The deterministic collapse operators used are acoustic mode loss ( $\sqrt{\Gamma}\hat{b}$ ), internal optical loss ( $\sqrt{\kappa^{\text{int}}}\hat{a}_h$ ), and detection inefficiency ( $\sqrt{(1 - \eta_d)\kappa^{\text{ex}}}\hat{a}_h$ ). The stochastic collapse operator is detection, including its efficiency ( $\sqrt{\eta_d\kappa^{\text{ex}}}\hat{a}_h$ ). To find the heralding probability, the number of simulations where the photodetector was triggered exactly once is divided by the total number of simulations. To find the heralding fidelity, the single-phonon component of the density matrix at the end of each simulation instance which heralded is averaged together. We only perform the simulation for the target parameter set.

We simulate the heralding process for squeezing drive peak powers  $P_b = 10 \mu\text{W}$  and  $P_b = 25, 50, \dots, 175 \mu\text{W}$ , and for detection efficiencies  $\eta_d = 0.80, 0.90, 0.95, 0.98$ , and  $0.99$ . Each point in Fig. 2 represents the average of 50,000 Monte Carlo trajectories. Dark counts are not directly simulated because it is not feasible to perform enough simulations to capture their effect with  $p_d = 4 \times 10^{-7}$ . Instead, the fidelity is adjusted after the simulation by  $F_h \rightarrow F_h p_h / (p_h + p_d(1 - p_h))$ .<sup>6</sup> This expression was validated by direct simulation of dark counts using  $p_d = 10^{-3}$  and  $p_d = 10^{-2}$ .

The time-dependence used for the Hamiltonian is  $\overline{\alpha_b} \sqrt{\tanh(f(t + \tau/2)) - \tanh(f(t - \tau/2))}$ , where  $\overline{\alpha_b} = \sqrt{4P_b/\hbar\kappa_b\omega_b}$  is the peak amplitude of the blue mode (the pulse does not actually reach this peak because it is too short),  $f = 3.8 \text{ ns}^{-1}$  is the speed at which the amplitude rises, and  $\tau = 1 \text{ ns}$  is the pulse’s FWHM. The pulse rise time is chosen to accurately reflect the build-up of energy in an optical resonator with the chosen external coupling rate ( $\kappa^{\text{ex}} \sim 1 \text{ GHz}$ ), and the pulse duration is kept short in order for the heralding cycle duration to be short when we consider parallelization (Sec. IID). The simulation starts at  $t = 0$ , the pulse is centered at  $t_0 = \tau/2 + 4.4/f \approx 1.66 \text{ ns}$ , and the simulation ends at  $2.5t_0 \approx 4.14 \text{ ns}$ .

<sup>6</sup>  $p_d$  ought to be multiplied by the probability of no detections,  $p_{a-h}$  (S64), rather than by  $(1 - p_h)$ , but the difference is negligible here.

## F. Heralded and anti-heralded phonon state

Above, we found the probability of having a single phonon given a herald in an imperfect system. By the same methodology, we can find the entire density matrix,  $\rho_h$ , of the acoustic mode conditioned on a successful herald. All coherence induced by the squeezing Hamiltonian is between the acoustic and optical mode, so the acoustic mode's density matrix is diagonal after tracing out the optical mode.

With  $\eta$  the total probability of detecting a generated photon as before, we find the probability to have  $k$  phonons after a successful herald using Bayes theorem:

$$\langle k | \rho_h | k \rangle = P(k \text{ phonons} | \text{herald}) = P(\text{herald} | k \text{ phonons}) \frac{P(k \text{ phonons})}{P(\text{herald})}. \quad (\text{S61})$$

Compare the above to Eq. (S57). Proceeding similarly,

$$\langle k | \rho_h | k \rangle = \begin{cases} p_d p_0 / p_h & k = 0 \\ p_0 \eta k (p_1 / p_0)^k (1 - \eta)^{k-1} / p_h & k > 0, \end{cases} \quad (\text{S62})$$

and the expected number of phonons is

$$\mathbb{E}[k | \text{herald}] = \langle \hat{b}^\dagger \hat{b} \rangle_h = F_{h,sp} \frac{(1 + (p_1/p_0)(1 - \eta))}{(1 - (p_1/p_0)(1 - \eta))^3}. \quad (\text{S63})$$

If dark counts are negligible, the phonon number distribution can be written  $\langle k | \rho_h | k \rangle = k F_{h,sp} (1 - \sqrt{F_{h,sp}})^{k-1}$ , and the expected number of phonons is  $\frac{2}{\sqrt{F_{h,sp}}} - 1$ .

We also consider the acoustic state given *no* detections at the herald frequency during the detection window, which we call an “anti-herald.” The anti-herald probability is

$$p_{a-h} = p_0 \left( (1 - p_d) + \frac{(p_1/p_0)(1 - \eta)}{1 - (p_1/p_0)(1 - \eta)} \right). \quad (\text{S64})$$

This is different from the probability of no herald  $1 - p_h$ , because  $1 - p_h$  includes the possibility of 2 or more detections. The density matrix after an anti-herald,  $\rho_{a-h}$ , is diagonal, with elements

$$\langle k | \rho_{a-h} | k \rangle = P(k \text{ phonons} | \text{anti-herald}) = \begin{cases} (1 - p_d) p_0 / p_{a-h} & k = 0 \\ p_0 (p_1/p_0)^k (1 - \eta)^k / p_{a-h} & k > 0, \end{cases} \quad (\text{S65})$$

which describes a thermal state with a slightly modified ground-state occupancy. The anti-heralded state has the expected number of phonons

$$\mathbb{E}[k | \text{anti-herald}] = \langle \hat{b}^\dagger \hat{b} \rangle_{a-h} = \frac{p_0}{p_{a-h}} \frac{(p_1/p_0)(1 - \eta)}{(1 - (p_1/p_0)(1 - \eta))^2}. \quad (\text{S66})$$

If dark counts are negligible, the anti-heralded state is a thermal state with  $\frac{1}{\sqrt{F_{h,sp}}} - 1 \approx \frac{1}{2}(1 - F_{h,sp})$  phonons.

## S5. RETRIEVAL OF A SINGLE PHOTON/OPTOMECHANICAL BEAM-SPLITTING

### A. Evolution of expectation values

In this section, we describe how the system evolves under optomechanical beam-splitting. The Hamiltonian of interest is Eq. (4), reproduced here:

$$\hat{H}_{bs} = g_0(\alpha_r^* \hat{a}_0 \hat{b}^\dagger + \alpha_r \hat{a}_0^\dagger \hat{b}).$$

Including both optical and acoustic loss and heating, we obtain equations of motion from the master equation:

$$\dot{n}_a = -g\sigma - \kappa n_a \quad (\text{S67})$$

$$\dot{n}_{\text{ph}} = g\sigma - \Gamma(n_{\text{ph}} - \bar{n}_{\text{ph}}) \quad (\text{S68})$$

$$\dot{\sigma} = 2g(n_a - n_{\text{ph}}) - (\kappa + \Gamma)\sigma/2, \quad (\text{S69})$$

where  $n_a = \langle \hat{a}_0^\dagger \hat{a}_0 \rangle$  is the photon population,  $n_{\text{ph}} = \langle \hat{b}^\dagger \hat{b} \rangle$  is the phonon population,  $\sigma = i\langle \hat{a}_0^\dagger \hat{b} - \hat{a}_0 \hat{b}^\dagger \rangle$ ,  $g = g_0 \alpha_r$ ,  $\bar{n}_{\text{ph}}$  is the phonon population at thermal equilibrium, and we have let  $\alpha_r = |\alpha_r|$ . If  $g$  is constant in time (continuous driving), and neglecting acoustic loss and heating ( $\Gamma \bar{n}_{\text{ph}} \approx 0$ ), the solution to these coupled differential equations is

$$\begin{aligned} n_0 &= (g/\zeta)^2 e^{-\kappa t/2} \sinh^2(\zeta t) n_{\text{ph}}(0), \\ n_{\text{ph}} &= e^{-\kappa t/2} \left( \cosh(\zeta t) + \frac{\kappa}{4\zeta} \sinh(\zeta t) \right)^2 n_{\text{ph}}(0), \\ \sigma &= 2(g/\zeta) e^{-\kappa t/2} \sinh(\zeta t) \left( \cosh(\zeta t) + \frac{\kappa}{4\zeta} \sinh(\zeta t) \right) n_{\text{ph}}(0) \end{aligned}$$

where  $\zeta = \sqrt{(\kappa_0/4)^2 - (g_0 \alpha_r)^2}$  is the effective coupling rate and  $n_{\text{ph}}(0) \approx 1$  is the initial phonon population. These solutions are used in Sec. II C.

### B. Beam-splitting as cooling

The slowest-decaying part of  $n_{\text{ph}}$  has rate

$$\Gamma_{\text{eff}}^\downarrow = (\kappa_0 + \Gamma)/2 - 2\zeta \approx \Gamma + 4|g\alpha_r|^2/(\kappa_0 - \Gamma) \approx \Gamma + \Gamma_{\text{opt}}^\downarrow. \quad (\text{S70})$$

The first approximation requires  $16|g\alpha_r|^2 \ll (\kappa_0 - \Gamma)^2$ , which is fulfilled if  $\kappa_0 \gg 4|g\alpha_r|, \Gamma$ ; and the second approximation requires  $\kappa_0 \gg \Gamma$ . This shows the validity of the effective cooling rate formulation, Eq. (S29), for moderate drive strength.

## S6. MINIMUM NECESSARY OM COUPLING RATE

In Sec. II F and Fig. 5 of the main text, we found the minimum OM coupling rate ( $g_0$ ) necessary to reach an average total single-photon fidelity of  $F_{\text{tot}} = 99\%$ . Below, we provide details of the calculation. In Fig. S3, we present the external optical coupling rate ( $\kappa^{\text{ex}}$ ), photon-phonon pair generation probability ( $p_1$ ), and the re-initialization drive duration ( $T_{\text{init}}$ ) which achieve this target when combined with the given  $g_0$ ,  $\eta_d$ ,  $n_{\text{th}}$ , and  $N$ .

The average total single-photon fidelity is  $F_{\text{tot}} = F_{\text{init}} F_{\text{h,sp}} F_{\text{idle}} \eta_{\text{re}}$  [Eq. (18)]. The parameter-dependent calculations of the idling fidelity ( $F_{\text{idle}}$ ) and retrieval efficiency ( $\eta_{\text{re}}$ ) are simple and described in full in the main text. The calculation of the single-phonon (SP) heralding fidelity ( $F_{\text{h,sp}}$ ) and initialization fidelity ( $F_{\text{init}}$ ) are described in more detail here. The parameters of the model are  $g_0$ ,  $\eta_d$ ,  $n_{\text{th}}$ ,  $N$ ,  $\kappa^{\text{ex}}$ ,  $p_1$ , and  $T_{\text{init}}$ . The internal optical loss is fixed at  $\kappa^{\text{int}} = 1$  MHz, and we use  $\kappa = \kappa^{\text{ex}} + \kappa^{\text{int}}$  for convenience in this section.

In Sec. S4 D, we derived Eq. (S60) for the SP heralding fidelity,  $F_{\text{h,sp}}$ . The variables in Eq. (S60) are the photon-phonon pair generation probability ( $p_1$ ), the probability of no photon-phonon pairs being generated ( $p_0$ ), the total efficiency ( $\eta$ ), and the detector dark count probability ( $p_d$ ). For the calculation of total single-photon fidelity in this section,  $p_1$  is a parameter of the model and  $p_0 = (1 + \sqrt{1 - 4p_1})/2$ . The total efficiency is  $\eta = \eta^{\text{ex}} \eta_d$ , where  $\eta^{\text{ex}} = \kappa^{\text{ex}}/\kappa$ . To determine the dark count probability,  $p_d$ , we must know the duration of the herald detection window. To this end, we calculate the necessary squeezing drive duration to reach the given photon-phonon pair generation probability using the short-time, constant-drive approximation for the phonon population:  $p_1 \approx n_{\text{ph}} \approx (g_0 \alpha_b t)^2$ , taking the classical drive power to be 1 mW. Note that the blue drive population,  $|\alpha_b|^2$ , depends on the total optical loss rate,  $\kappa$ . If the calculated squeezing drive duration is shorter than the cavity response time  $2\pi/\kappa$ , we set the drive duration to be  $2\pi/\kappa$  and suppose it has a lower power. We take the squeezing drive duration, plus another  $2 \times 2\pi/\kappa$  to allow for any generated herald photons to escape, to be the duration of the herald detection window. This duration is multiplied by the dark count rate 100 c.p.s. to find the dark count probability,  $p_d$ .

The initialization fidelity,  $F_{\text{init}} \approx 1 - n_{\text{ph}}$ , is the ground-state occupancy of the acoustic mode after cooling. For the dynamics of the phonon mode under cooling, we use the simple expressions in Sec. S2 A. When no drives are applied,

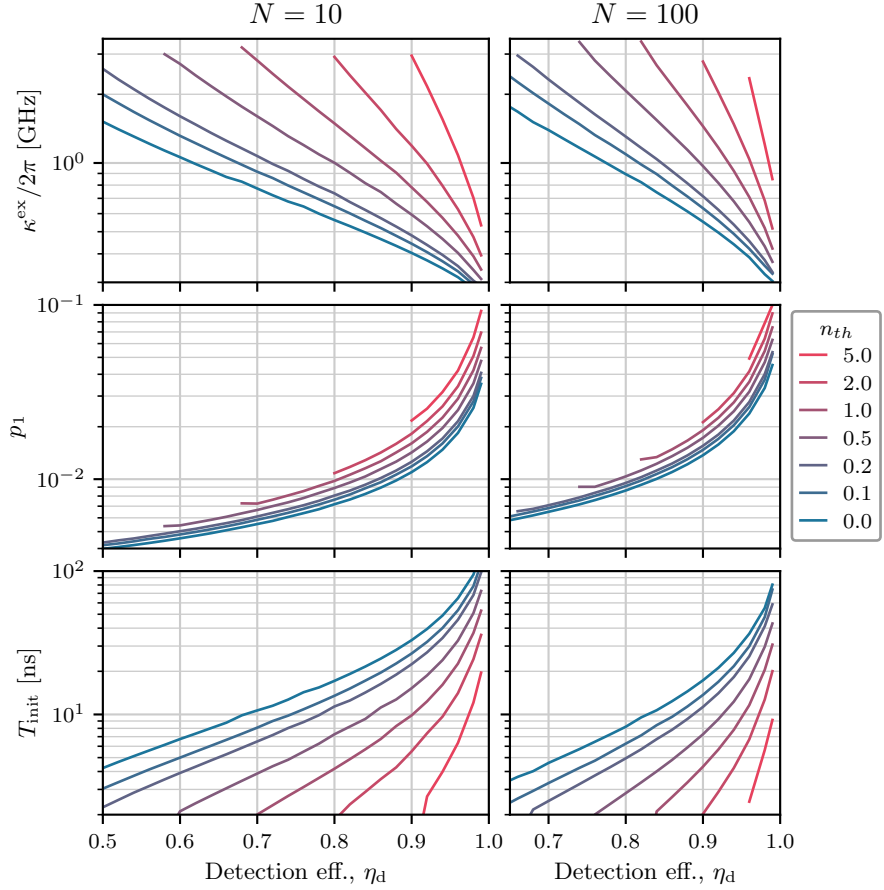

FIG. S3. Optimized external optical coupling rate ( $\kappa^{\text{ex}}$ ), photon-phonon pair generation probability ( $p_1$ ), and the re-initialization drive duration ( $T_{\text{init}}$ ) which reach 99% total single-photon fidelity when combined with the given detection efficiency ( $\eta_d$ ), thermal phonon population ( $n_{th}$ ), number of OM systems ( $N$ ), and OM coupling rate ( $g_0$ ) given in Fig. 5.

the acoustic mode loses phonons at the rate  $\Gamma_{\text{th}}^{\downarrow} = (n_{\text{th}} + 1)\Gamma$  and gains phonons at the rate  $\Gamma_{\text{th}}^{\uparrow} = n_{\text{th}}\Gamma$ . Under a constant beam-splitting drive, the phonon population decays through the optical mode at rate  $\Gamma_{\text{opt}}^{\downarrow} = \frac{4g_0^2|\alpha_r|^2}{\kappa_0}$ , giving a total decay rate of  $\Gamma_{\text{tot}}^{\downarrow} = \Gamma_{\text{th}}^{\downarrow} + \Gamma_{\text{opt}}^{\downarrow}$ . Let  $n_1$  be the phonon population at the beginning of the re-initialization drive. We integrate the phonon population equation of motion ( $\dot{n}_{\text{ph}} = -\Gamma_{\text{tot}}^{\downarrow}n_{\text{ph}} + \Gamma_{\text{tot}}^{\uparrow}(n_{\text{ph}} + 1)$ ), to find the phonon population after the drive:

$$n_0 = n_1 e^{-\Gamma_{\text{net}}^{\downarrow} T_{\text{init}}} + \frac{\Gamma_{\text{th}}^{\uparrow}}{\Gamma_{\text{net}}^{\downarrow}} \left(1 - e^{-\Gamma_{\text{net}}^{\downarrow} T_{\text{init}}}\right), \quad (\text{S71})$$

where  $\Gamma_{\text{net}}^{\downarrow} = \Gamma_{\text{tot}}^{\downarrow} - \Gamma_{\text{th}}^{\uparrow}$ . If no herald photon is detected during the squeezing portion of the next heralding cycle,  $n_{\text{add}} = 1/\sqrt{F_{\text{h,sp}}} - 1$  phonons are added to the acoustic mode (see Sec. S4F). The acoustic mode thermalizes while the beam-splitting drive is not active. Therefore, the phonon population at the beginning of the next re-initialization drive is

$$n'_1 = (n_0 + n_{\text{add}}) e^{-\Gamma(T_{\text{h}} - T_{\text{init}})} + n_{\text{th}} \left(1 - e^{-\Gamma(T_{\text{h}} - T_{\text{init}})}\right). \quad (\text{S72})$$

We solve Eqs. (S71)–(S72) to find the fixed-point value of  $n_0$ , and use  $F_{\text{init}} = 1 - n_0$  for results in this section and Sec. IIF.

## S7. COMPARISON OF PARALLELIZED OM SINGLE-PHOTON SOURCE TO OTHER SINGLE PHOTON SOURCES

The proposed optomechanical single-photon source is inspired by all-optical photon-pair sources (e.g. based on spontaneous parametric down-conversion) which may be multiplexed to reliably produce single photons. The advantage of the scheme presented here, relative to all-optical photon-pair sources, lies in the separation of the preparation

and retrieval phases. Instead of requiring fast routing of heralded single photons, the single phonon is automatically preserved in place and can be read out on demand. The single-photon fidelity decays according to  $e^{-(3n_{\text{th}}+1)\Gamma t}$  while idling (Sec. IID). Assuming a base temperature of 2 K ( $n_{\text{th}} = 3.7$ ), the fidelity of the acoustic mode to the single-phonon state degrades by 7.6 ppm per 10-ns heralding cycle, only reaching 1% degradation after 1,320 heralding cycles, using the target parameter set. This allows one to reach very high levels of multiplexing without extra engineering. High levels of multiplexing are desirable because they allow one to decrease the heralding probability per cycle, improving the heralding fidelity (Sec. IIB). On the other hand, for the near-term parameter set,  $n_{\text{th}} = 2.7$  at 2 K, and the single-phonon state degrades by 572 ppm per 200 ns heralding cycle, reaching 1% degradation after 17 cycles. This could be improved by shortening the heralding cycle duration by allowing stronger optical drives than 1 mW.

We now return our focus to the target parameter set. To concretely compare this scheme to a traditional all-optical scheme, suppose we wish to multiplex 1,024 spatio-temporal modes of heralded single-photon sources into one reliable single-photon source. The proposed optomechanical single-photon source experiences 0.77% loss of fidelity over 1,024 heralding cycles. Three possible optical multiplexing architectures are considered—the log tree, which minimizes the total optical switch depth; the generalized Mach-Zehnder interferometer, which minimizes optical phase modulator depth; and the storage loop, which is the simplest and most flexible architecture. See [9] for illustrations of the log tree and GMZI architectures, and [10] for an overview of experimental progress building such multiplexers. Using a log tree architecture, each optical mode must pass through ten  $2\times 1$  switches (typically Mach-Zehnder interferometers with tunable phase modulators), requiring each switch to have no more than 0.078% loss to achieve the same total loss of fidelity as the optomechanical source. With a generalized Mach-Zehnder interferometer, the modes only pass through one phase modulator but a prodigious 2,046  $2\times 2$  couplers, requiring each coupler to have less than 3.8 ppm loss. Finally, we consider a storage loop architecture such as demonstrated in [11, 12], which is directly analogous to this proposal, and therefore would need to reach 7.6 ppm loss per cycle to be capable of the same level of multiplexing while maintaining the same level of fidelity as the optomechanical source. This shows that the proposed system allows one to achieve levels of multiplexing not attainable in all-optical schemes.

The proposed optomechanics-based single-photon source lends itself to asynchronous operation, outputting sets of single photons as they become available rather than on a fixed schedule. As outlined in [13], this “relative” multiplexing allows more efficient use of resources by allowing one to extract sets of photons early when they happen to be produced early. However, when using all-optical relative multiplexing, one must still build a substantial set of optical delay lines to accommodate instances when the photons are produced far apart in time. No such unwieldy system is required for the optomechanical single-photon source.

Another advantage of the proposed system, as compared to parametric photon-pair sources, arises from the great difference between the linewidths of the optical and acoustic modes. In parametric photon-pair production, the signal and idler photons will be spectrally entangled, unless one takes steps to avoid it [14]. Such signal-idler entanglement is detrimental because either one photon is projected onto a mixed state when the other is detected as a herald, or one must spectrally filter the single photons, introducing loss. In contrast, the narrow linewidth of the acoustic phonon ensures that any output single photons will simply inherit the spectral properties of the optical drive and will not be spectrally entangled with the phonon. This enables the experimentalist to adjust the optical drive strength and duration without sacrificing indistinguishability.

The proposed system is more flexible and tailorable than quantum dot and other deterministic sources of single photons. Despite experimental progress, matter-based sources still suffer from inadequate extraction efficiency and poor indistinguishability [15–17]. Furthermore, many such sources operate in the visible regime, necessitating quantum frequency conversion to telecom wavelengths to access state-of-the-art tools and integrated photonics platforms [18].

One challenge of the proposed optomechanical system is it must be operated at cryogenic temperatures. Another issue is the latency of the heralding feedback, by which we mean the time between the determination of whether the system heralded (the right edges of the blue boxes in Fig. 3) and when the red drive is turned on to reset the phononic system to the ground state (the left edges of the red boxes in Fig. 3). The latency of the heralding feedback must be faster than the generation clock cycle. The feedback cycle on an all-optical photon-pair generation system may have high latency while maintaining high throughput because each potential pair of photons occupies a different temporal mode. In contrast, extra phonons generated in this scheme will occupy the same mode as the original phonon due to the mode’s stationary nature and low loss. Despite these drawbacks, we believe this scheme offers a promising avenue for generating single photons for linear optical quantum computing.

## S8. ERROR LIFETIMES OF PHONONIC DUAL-RAIL QUBITS

The leakage lifetime,  $\tau_1$ , is defined as the inverse of the rate at which the phononic qubit leaves the dual-rail subspace:  $\Gamma\tau_1 = 1/(4n_{\text{th}} + 1)$ , where  $n_{\text{th}}$  is the thermal phonon population. The contributions to the leakage rate are

$n_{\text{th}}\Gamma$  for heating out of the ground state,  $(n_{\text{th}} + 1)\Gamma$  for cooling out of Fock  $|1\rangle$ , and  $2n_{\text{th}}\Gamma$  for heating out of  $|1\rangle$ . At low temperatures ( $n_{\text{th}} \ll 1$ ),  $\tau_1$  is the time when the probability of being in the dual-rail subspace falls to  $1/e$  of its original value.

The bit flip lifetime,  $\tau_X$ , is defined as the time when the probability of a bit flip within the dual-rail subspace crosses  $1/2e$ . To find an analytical expression, we calculate the evolution of each mode as it thermalizes, restricted to the  $|n \leq 1\rangle$  subspace. Supposing we started in the  $|01\rangle$  state (Fock basis), the probability of a bit flip is  $P(|10\rangle)/(P(|01\rangle) + P(|10\rangle))$ , where  $P(|\psi\rangle) = \langle\psi|\rho(t)|\psi\rangle$ . This gives the bit-flip lifetime

$$\Gamma\tau_X = \tanh(\beta\Omega/2) \log \left\{ 1 + \frac{1}{(e-1)} \cosh^2(\beta\Omega/2) \left( 1 + \sqrt{1 + 2(e-1) \text{sech}^2(\beta\Omega/2)} \right) \right\}, \quad (\text{S73})$$

where  $\beta = (k_B T)^{-1}$ ,  $k_B$  is the Boltzmann constant and  $T$  is the phonon bath temperature. Despite the subspace restriction, this formula agrees with numerical simulations for the entire temperature range considered, up to  $T = 12$  K,  $n_{\text{th}} \approx 25$ .

A variety of simulations are used to validate these analytical expressions. Leakage lifetimes are calculated by QuTiP master equation simulations up to 500 mK and by custom Monte Carlo simulations for 600 mK and above. Our Monte Carlo simulation is untruncated, allowing for arbitrarily high number states. Bit-flip lifetimes are calculated by restricted-subspace analytical approximation for 40-80 mK, by master equation simulation for 100-500 mK, and by our Monte Carlo simulation for 600 mK and above. MC results match ME results where they are both available.

## S9. SINGLE-SHOT GHZ-STATE PREPARATION IN PHONONIC MEMORIES

In this section we describe the GHZ-state preparation protocol from Sec. IIIB of the main text in more detail. In Sec. S9 A–S9 D, we prove that the heralding probability ( $p_{\text{h,ghz}}$ ) and fidelity ( $F_{\text{h,ghz}}$ ) are given by Eq. (22)–(23), reproduced here:

$$p_{\text{h,ghz}} = 2(\eta p_{\text{re}})^n (1 - \eta p_{\text{re}})^n \left( 1 + n^2 p_{\text{d}} \frac{1 - \eta p_{\text{re}}}{\eta p_{\text{re}}} \right), \quad (\text{S74})$$

$$F_{\text{h,ghz}} = \left( \frac{1 - p_{\text{re}}}{1 - \eta p_{\text{re}}} \right)^n \left( 1 + n^2 p_{\text{d}} \frac{1 - \eta p_{\text{re}}}{\eta p_{\text{re}}} \right)^{-1}. \quad (\text{S75})$$

These account for optical loss ( $\eta < 1$ ) and the possibility of a single detector dark count ( $n p_{\text{d}} \ll \eta p_{\text{re}}$ ). Section S9 E describes the simulation which validates these expressions.

We use the same notation as in the main text, unless otherwise noted: acoustic modes are grouped into pairs which are indexed by  $i \in \{1, 2, \dots, n\}$ . Within each pair the modes are labeled by  $q \in \{0, 1\}$ . Therefore, each acoustic mode has a unique label  $[i, q]$ . Each acoustic mode is coupled to its own optical mode which shares the same label,  $[i, q]$ .

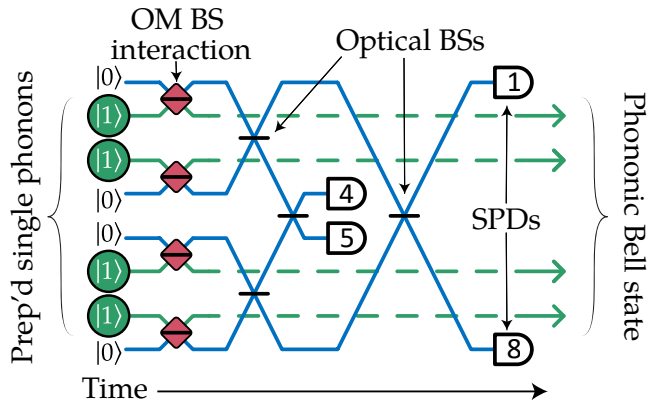

FIG. S4. Linearized optomechanical protocol for preparing a Bell state in the acoustic modes, same as Fig. 7, in conventional optical notation. Note detectors are numbered differently. Blue lines correspond to optical modes while green lines represent acoustic modes.

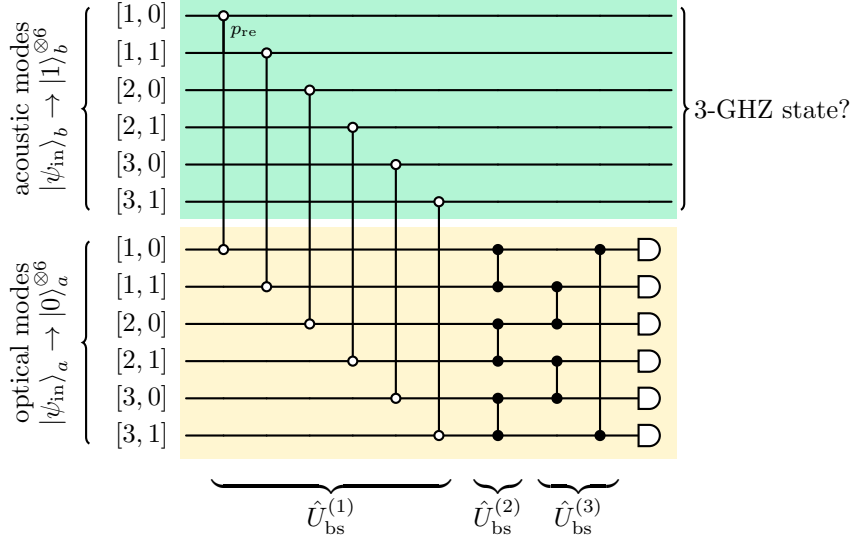

FIG. S5. **Protocol for preparing 3-GHZ state with optomechanics.** Expanded version of Fig. 7. As there, each horizontal wire represents a mode (acoustic or optical), vertical lines with solid endpoints represent 50/50 beam splitters, and vertical lines with open endpoints represent tunable beam splitters (tuning parameter  $p_{\text{re}}$ ). The protocol has three stages of beam-splitting followed by detection of the optical modes.

### A. GHZ-state heralding in an ideal system

Here we show that the protocol described in Sec. III B produces the states  $|n\text{-GHZ}^\pm\rangle = (|+\rangle^{\otimes n} \pm |-\rangle^{\otimes n})/\sqrt{2}$  with heralding probability  $2p_{\text{re}}^n(1-p_{\text{re}})^n$  in an ideal system. The scheme is illustrated in Figs. 7 and S4 for  $n=2$  and in Fig. S5 for  $n=3$ . For convenience, we define the generic beam-splitting unitary

$$\hat{U}_{\text{bs}}[\hat{a}, \hat{b}; t] = \exp\left(\theta(\hat{a}\hat{b}^\dagger - \hat{a}^\dagger\hat{b})\right), \quad (\text{S76})$$

which gives

$$\begin{aligned} \hat{U}_{\text{bs}}[\hat{a}, \hat{b}; t] \hat{a} \hat{U}_{\text{bs}}^\dagger[\hat{a}, \hat{b}; t] &= r\hat{a} + t\hat{b}, & \hat{U}_{\text{bs}}^\dagger[\hat{a}, \hat{b}; t] \hat{a} \hat{U}_{\text{bs}}[\hat{a}, \hat{b}; t] &= r\hat{a} - t\hat{b}, \\ \hat{U}_{\text{bs}}[\hat{a}, \hat{b}; t] \hat{b} \hat{U}_{\text{bs}}^\dagger[\hat{a}, \hat{b}; t] &= r\hat{b} - t\hat{a}, & \hat{U}_{\text{bs}}^\dagger[\hat{a}, \hat{b}; t] \hat{b} \hat{U}_{\text{bs}}[\hat{a}, \hat{b}; t] &= r\hat{b} + t\hat{a}, \end{aligned}$$

where  $r = \cos \theta$  and  $t = \sin \theta$  are the beam splitter reflection and transmission amplitude, respectively. When no  $t$  is given, assume  $t = 1/\sqrt{2}$ . With this notation, the beam-splitting part of the OM protocol to prepare an  $n$ -GHZ state is

$$\hat{U}_{\text{tot}} = \underbrace{\left(\prod_{i=1}^n \hat{U}_{\text{bs}}[\hat{a}_{[i,1]}, \hat{a}_{[i+1,0]}\right]}_{\hat{U}_{\text{bs}}^{(3)}} \underbrace{\left(\prod_{i=1}^n \hat{U}_{\text{bs}}[\hat{a}_{[i,0]}, \hat{a}_{[i,1]}\right]}_{\hat{U}_{\text{bs}}^{(2)}} \underbrace{\left(\prod_{i=1}^n \prod_{q \in \{0,1\}} \hat{U}_{\text{bs}}[\hat{b}_{[i,q]}, \hat{a}_{[i,q]}; t]\right)}_{\hat{U}_{\text{bs}}^{(1)}}, \quad (\text{S77})$$

where  $\hat{a}_{[i,q]}$  are the optical mode operators and  $\hat{b}_{[i,q]}$  are the acoustic mode operators (see Fig. S5). We let  $t = \sqrt{p_{\text{re}}}$  in  $\hat{U}_{\text{bs}}^{(1)}$ . The mode-pair labels,  $i$ , are restricted to 1 through  $n$ , periodically. That is, the  $n$ th term in the product  $\hat{U}_{\text{bs}}^{(3)}$  is  $\hat{U}_{\text{bs}}[\hat{a}_{[n,1]}, \hat{a}_{[1,0]}]$ . Topologically speaking, the mode pairs are connected in a ring. The initial state is  $|\Psi_{\text{in}}\rangle_{ab} = |\psi_{\text{in}}\rangle_a |\psi_{\text{in}}\rangle_b = |0\rangle_a^{\otimes 2n} |1\rangle_b^{\otimes 2n}$ , with subscripts indicating whether the state is defined on the optical modes ( $a$ ), the acoustic ( $b$ ) modes, or both ( $ab$ ). For describing the detection patterns, we introduce an alternate labelling for the optical modes,  $\hat{d}_{[i,s_i]}$  ( $d$  for “detected”), where  $s_i \in \{+1, -1\}$ , defining  $\hat{d}_{[i,+]} := \hat{a}_{[i,1]}$  and  $\hat{d}_{[i,-]} := \hat{a}_{[i+1,0]}$ . A GHZ-herald detection pattern can be described by the  $n$  parity bits,  $\{s_i\}$ .

We now calculate the state of the acoustic modes after a herald detection. The optical modes must be in vacuum after detection. Therefore, the (unnormalized) state of the acoustic modes after heralding is

$$|\psi_{\text{f}}\rangle_b = \langle 0|_a^{\otimes 2n} |\Psi_{\text{f}}\rangle_{ab} = \langle 0|_a^{\otimes 2n} \left(\prod_{i=1}^n \hat{d}_{[i,s_i]}\right) \hat{U}_{\text{tot}} |\Psi_{\text{in}}\rangle_{ab}. \quad (\text{S78})$$

Notice that we remove the optical modes from the final expression by collapsing that subsystem onto the vacuum state. This is similar to taking a partial trace to remove those modes, but it leaves the acoustic modes in pure state. To evaluate Eq. (S78), we commute the beam-splitting operators to the left, noting that  $\langle 0|_a^{\otimes 2n} \hat{U}_{\text{bs}}^{(3)} = \langle 0|_a^{\otimes 2n} \hat{U}_{\text{bs}}^{(2)} = \langle 0|_a^{\otimes 2n}$ :

$$\begin{aligned} |\psi_f\rangle &= \langle 0|_a^{\otimes 2n} \left( \prod_{i=1}^n \hat{d}_{[i,s_i]} \right) \hat{U}_{\text{bs}}^{(3)} \hat{U}_{\text{bs}}^{(2)} \hat{U}_{\text{bs}}^{(1)} |0\rangle_a^{\otimes 2n} |1\rangle_b^{\otimes 2n} \\ &= \frac{1}{2^n} \langle 0|_a^{\otimes 2n} \prod_{i=1}^n [(\hat{a}_{[i,0]} + \hat{a}_{[i,1]}) - s_i(\hat{a}_{[i+1,0]} - \hat{a}_{[i+1,1]})] \hat{U}_{\text{bs}}^{(1)} |0\rangle_a^{\otimes 2n} |1\rangle_b^{\otimes 2n} \\ &= \frac{t^n}{2^{n/2}} \langle 0|_a^{\otimes 2n} \hat{U}_{\text{bs}}^{(1)} |0\rangle_a^{\otimes 2n} \prod_{i=1}^n (\hat{b}_{[i,+]} - s_i \hat{b}_{[i+1,-]}) |1\rangle_b^{\otimes 2n}, \end{aligned} \quad (\text{S79})$$

where  $\hat{b}_{[i,\pm]} = (\hat{b}_{[i,0]} \pm \hat{b}_{[i,1]})/\sqrt{2}$ . Now we evaluate  $\langle 0|_a^{\otimes 2n} \hat{U}_{\text{bs}}^{(1)} |0\rangle_a^{\otimes 2n}$  by inserting a projector onto optical vacuum (which has no effect), using a resolution of the identity on the acoustic modes, and using the definition of  $\hat{U}_{\text{bs}}^{(1)}$ :

$$\begin{aligned} \langle 0|_a^{\otimes 2n} \hat{U}_{\text{bs}}^{(1)} |0\rangle_a^{\otimes 2n} &= \langle 0|_a^{\otimes 2n} \prod_{i,q} \left\{ \left( |0\rangle\langle 0|_{a,[i,q]} \otimes \hat{I}_{b,[i,q]} \right) \hat{U}_{\text{bs}} \left[ \hat{b}_{[i,q]}, \hat{a}_{[i,q]}; t \right] \right\} |0\rangle_a^{\otimes 2n} \\ &= \langle 0|_a^{\otimes 2n} \prod_{i,q} \left\{ \sum_{m=0}^{\infty} \frac{1}{m!} (\hat{b}_{[i,q]}^\dagger)^m |00\rangle\langle 00|_{ab,[i,q]} (r \hat{b}_{[i,q]})^m \right\} |0\rangle_a^{\otimes 2n} \\ &= r^{\hat{n}_{\text{ph}}} \end{aligned} \quad (\text{S80})$$

where  $\hat{n}_{\text{ph}} = \sum_{i,q} \hat{b}_{[i,q]}^\dagger \hat{b}_{[i,q]}$  is the total number of phonons. The final step can be seen by writing  $r^{\hat{b}_{[i,q]}^\dagger \hat{b}_{[i,q]}}$  in the number basis. Combing Eqs. (S79) and (S80), we have

$$|\psi_f\rangle = \overbrace{\frac{t^n}{2^{n/2}} r^{\hat{n}_{\text{ph}}} \prod_{i=1}^n (\hat{b}_{[i,+]} - s_i \hat{b}_{[i+1,-]})}^{\mathbb{K}_{\text{GHZ}}^{\{s_i\}}, \text{ Eq. 20}} |1\rangle_b^{\otimes 2n} \quad (\text{S81})$$

$$= \frac{t^n}{2^{n/2}} r^{\hat{n}_{\text{ph}}} \left( \prod_{i=1}^n \hat{b}_{[i,+]} + \prod_{i=1}^n (-s_i \hat{b}_{[i+1,-]}) \right) |1\rangle_b^{\otimes 2n} \quad (\text{S82})$$

$$\begin{aligned} &= \frac{(rt)^n}{2^{n/2}} \left( |+_L\rangle_b^{\otimes n} + \bar{s} |-_L\rangle_b^{\otimes n} \right) \\ &= \frac{(rt)^n}{2^{n/2}} \sqrt{2} |n\text{-GHZ}^{\bar{s}}\rangle, \end{aligned} \quad (\text{S83})$$

where  $\bar{s} = \prod_{i=1}^n s_i$  is the parity of the final GHZ state, and we used  $\hat{b}_{[i,+]} \hat{b}_{[i,-]} |11\rangle_{b,i} = 0$ . This state has norm  $2(rt)^{2n}/2^n$ . Multiplying by the  $2^n$  possible herald detection patterns and replacing  $t = \sqrt{p_{\text{re}}}$  gives the heralding probability  $p_{\text{h,ghz}} = 2p_{\text{re}}^n (1 - p_{\text{re}})^n$  in the ideal case.

## B. GHZ-state overlap with acoustic modes

To calculate the GHZ-state heralding fidelity using Bayes' theorem (Eq. (21)), we require the unconditioned probability of the acoustic modes being in a GHZ state. This probability is the square-overlap between an ideal GHZ state and the state of the acoustic modes at the end of all beam-splitting rounds, irrespective of detection outcome (Fig. S5). Optical beam-splitting and optical loss do not affect this acoustic-mode overlap. Therefore, the unconditioned probability of the acoustic modes being in a GHZ state is

$$P(\text{GHZ state}) := \left| \langle n\text{-GHZ}^\pm |_b \hat{U}_{\text{bs}}^{(1)} |\Psi_{\text{in}}\rangle_{ab} \right|^2, \quad (\text{S84})$$

where  $\hat{U}_{\text{bs}}^{(1)}$  is the optomechanical beam-splitting unitary (see Eq. (S77)). This square-overlap is  $(rt)^{2n}$  for each of the 2 GHZ states. Thus, the total probability that the acoustic modes are in a GHZ state after the optomechanical beam splitter is  $2(rt)^{2n} = 2p_{\text{re}}^n(1 - p_{\text{re}})^n$ . The fact that this matches the heralding probability in an ideal system indicates that we have captured all possible heralding detection patterns.

### C. Probability of an arbitrary detection pattern with inefficient detectors

We calculate the relationship between the probability of a detection outcome with and without optical loss. This probability is used to calculate the GHZ-state heralding fidelity using Bayes' theorem. We show that, in general, the probability of a particular detection outcome when including optical loss can be found from the probability of that detection outcome neglecting loss by rescaling the retrieval probability  $p_{\text{re}} \rightarrow \eta p_{\text{re}}$ . For example, the probability of heralding an  $n$ -GHZ state in an ideal system is  $2p_{\text{re}}^n(1 - p_{\text{re}})^n$ , as shown in Sec. S9 A, so the heralding probability including optical loss is  $2(\eta p_{\text{re}})^n(1 - \eta p_{\text{re}})^n$ . This can be understood by considering a ballistic model of optical beam-splitting: in the ideal case, every photon which is detected must have been converted from a phonon, which occurs with probability  $p_{\text{re}}$ . On the other hand, when there is optical loss, every photon which is detected must have been converted from a phonon *and not lost*, which occurs with probability  $\eta p_{\text{re}}$ .

We provide a general proof for  $N$  acoustic modes numbered 1 through  $N$  and arbitrary optical beam splitting, see Fig. S6. In this subsection only, we label the modes instead of the mode pairs for brevity and generality. The initial state in the acoustic modes is  $|\psi_{\text{in}}\rangle_b$  and the detection pattern is given by the list of numbers  $\{\nu_i\} = \{\nu_1, \nu_2, \dots, \nu_N\}$ . The many-mode optical beam-splitting is described by a unitary  $\tilde{U}_a$ , defined by the real, unitary,  $N \times N$  matrix  $f$ :

$$\tilde{U}_a^\dagger \hat{a}_i \tilde{U}_a = \sum_{j=1}^N f_{ij} \hat{a}_j. \quad (\text{S85})$$

In the specific case of single-shot  $n$ -GHZ-state preparation as described in the previous subsection, the total number of modes is  $N = 2n$ , the initial state in the acoustic modes is  $|\psi_{\text{in}}\rangle_b = |1\rangle_b^{\otimes 2n}$ , and the optical beam-splitting unitary is  $\tilde{U}_a = U_{\text{bs}}^{(3)} U_{\text{bs}}^{(2)}$ . An example of a herald detection pattern used in Sec. S9 A is  $\{s_i\} = \{+, +, \dots, +\}$  (see definition of notation above Eq. (S78)), or  $\{\nu_i\} = \{0, 1, 0, 1, \dots, 0, 1\}$  in the notation of this subsection.

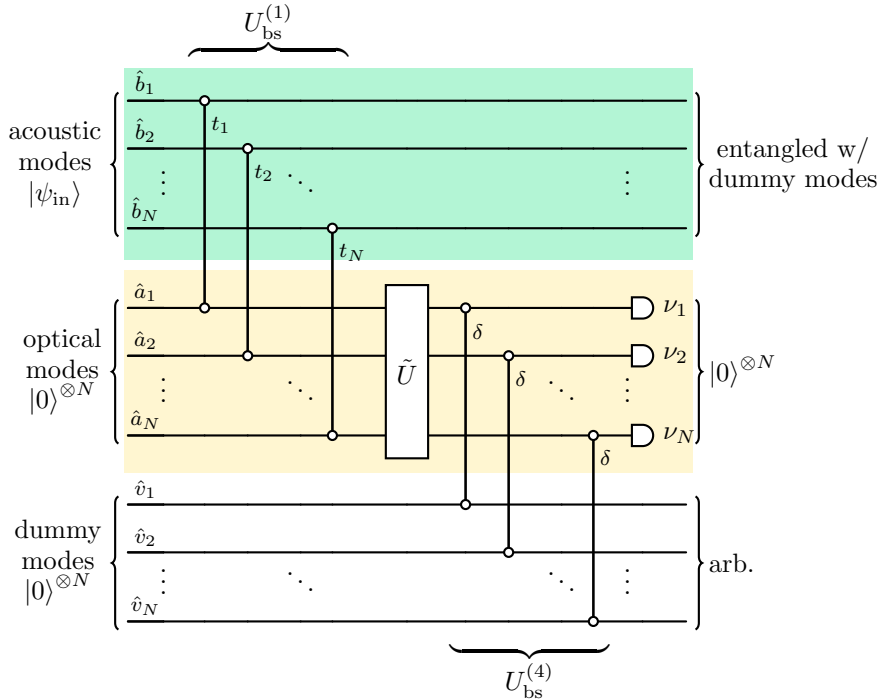

**FIG. S6. Introduce dummy modes to calculate detection probability with lossy detectors.** The dummy optical modes,  $\hat{v}_i$ , start in the vacuum state and end in an arbitrary state, entangled with the acoustic modes. The beam-splitting amplitude between the “real” optical modes,  $\hat{a}_i$ , and the dummy modes is  $\delta = \sqrt{1 - \eta}$ , where  $\eta$  is the detection system efficiency. Note that in this diagram we label beam splitters by their amplitude rather than their probability. The single photon detector on optical mode  $i$  detects  $\nu_i$  photons.

First, we calculate the detection probability using this generic setup but with no optical loss, i.e.,  $\eta = 1$ ,  $\delta = 0$ . This is a generalization of Sec. S9 A, except that we only calculate the detection probability in this section, and not

the final state. The final (unnormalized) state of OM system is

$$|\Psi_f\rangle_{ab} = \hat{K}_{\{\nu_i\}} \tilde{U}_a \hat{U}_{bs}^{(1)} |\Psi_{in}\rangle_{ab}, \quad (\text{S86})$$

where  $|\Psi_{in}\rangle_{ab} = |0\rangle_a^{\otimes N} |\psi_{in}\rangle_b$  is the initial state of the OM system,  $\hat{U}_{bs}^{(1)} = \prod_{i=1}^N \hat{U}_{bs} [\hat{b}_i, \hat{a}_i; t_i]$  is the OM beam-splitting unitary (Eq. S76), and  $\hat{K}_{\{\nu_i\}} = |0\rangle\langle 0|_a^{\otimes N} \prod_{i=1}^N \frac{1}{\sqrt{\nu_i!}} \hat{a}_i^{\nu_i}$  is the Kraus operator for the detection pattern  $\{\nu_i\}$ . Equation (S78) is a special case of Eq. (S86) with optical beam-splitting  $\tilde{U}_a \rightarrow \hat{U}_{bs}^{(3)} \hat{U}_{bs}^{(2)}$  and detection Kraus operator  $\hat{K}_{\{\nu_i\}} \rightarrow |0\rangle\langle 0|_a^{\otimes 2n} \prod_{i=1}^n \hat{d}_{i,s_i}$ .

To evaluate Eq. (S86), we expand  $\hat{K}_{\{\nu_i\}}$  and commute all unitary operators to the left:

$$\begin{aligned} |\Psi_f\rangle_{ab} &= |0\rangle\langle 0|_a^{\otimes N} \left[ \prod_{i=1}^N \frac{1}{\sqrt{\nu_i!}} \hat{a}_i^{\nu_i} \right] \tilde{U}_a \hat{U}_{bs}^{(1)} |\Psi_{in}\rangle_{ab} \\ &= |0\rangle\langle 0|_a^{\otimes N} \hat{U}_{bs}^{(1)} \left[ \prod_{i=1}^N \frac{1}{\sqrt{\nu_i!}} \left( \sum_{j=1}^N f_{ij} (r_j \hat{a}_j + t_j \hat{b}_j) \right)^{\nu_i} \right] |0\rangle_a^{\otimes N} |\psi_{in}\rangle_b \\ &= \left[ \prod_{i=1}^N r_i^{\hat{b}_i^\dagger \hat{b}_i} \right] \left[ \prod_{i=1}^N \frac{1}{\sqrt{\nu_i!}} \left( \sum_{j=1}^N f_{ij} t_j \hat{b}_j \right)^{\nu_i} \right] |0\rangle_a^{\otimes N} |\psi_{in}\rangle_b, \end{aligned}$$

where we used  $\langle 0|_a^{\otimes N} \hat{U}_{bs}^{(1)} |0\rangle_a^{\otimes N} = \prod_{i=1}^N r_i^{\hat{b}_i^\dagger \hat{b}_i}$  for the last line (see Eq. (S80)). Notice that the terms within each product commute. Therefore, the probability of getting detection pattern  $\{\nu_i\}$  is

$$P_{\{\nu_i\}}(\{t_i\}) := \langle \Psi_f | \Psi_f \rangle_{ab} = \langle \psi_{in} |_b \left[ \prod_{i=1}^N \frac{1}{\sqrt{\nu_i!}} \left( \sum_{j=1}^N f_{ij} t_j \hat{b}_j^\dagger \right)^{\nu_i} \right] \left[ \prod_{i=1}^N r_i^{2\hat{b}_i^\dagger \hat{b}_i} \right] \left[ \prod_{i=1}^N \frac{1}{\sqrt{\nu_i!}} \left( \sum_{j=1}^N f_{ij} t_j \hat{b}_j \right)^{\nu_i} \right] |\psi_{in}\rangle_b. \quad (\text{S87})$$

We include loss by introducing a set of dummy modes  $\hat{v}_i$ . Each “real” optical mode,  $\hat{a}_i$ , is beam-split with its corresponding dummy optical mode,  $\hat{v}_i$ , with beam-splitting amplitude  $\delta = \sqrt{1-\eta}$ , before being sent to a number-resolving single-photon detector (see Fig. S6). The unitary describing this beam-splitting is  $\hat{U}_{bs}^{(4)} = \prod_{i=1}^N \hat{U}_{bs} [\hat{a}_i, \hat{v}_i; \delta]$ . The dummy modes start in vacuum, so the initial state of the total system is  $|\Psi'_{in}\rangle_{vab} = |0\rangle_v^{\otimes N} |0\rangle_a^{\otimes N} |\psi_{in}\rangle_b$ . Therefore, the final state of the total system is

$$\begin{aligned} |\Psi'_f\rangle_{vab} &= \hat{K}_{\{\nu_i\}} \hat{U}_{bs}^{(4)} \tilde{U}_a \hat{U}_{bs}^{(1)} |\Psi'_{in}\rangle_{vab} \\ &= |0\rangle\langle 0|_a^{\otimes N} \hat{U}_{bs}^{(4)} \tilde{U}_a \hat{U}_{bs}^{(1)} \left[ \prod_{i=1}^N \frac{1}{\sqrt{\nu_i!}} \left( \sqrt{\eta} \left( \sum_{j=1}^N f_{ij} (r_j \hat{a}_j + t_j \hat{b}_j) \right) - \delta \hat{v}_i \right)^{\nu_i} \right] |0\rangle_v^{\otimes N} |0\rangle_a^{\otimes N} |\psi_{in}\rangle_b \\ &= |0\rangle\langle 0|_a^{\otimes N} \hat{U}_{bs}^{(4)} |0\rangle\langle 0|_v^{\otimes N} \tilde{U}_a \hat{U}_{bs}^{(1)} \left[ \prod_{i=1}^N \frac{1}{\sqrt{\nu_i!}} \left( \sqrt{\eta} \sum_{j=1}^N f_{ij} t_j \hat{b}_j \right)^{\nu_i} \right] |0\rangle_v^{\otimes N} |0\rangle_a^{\otimes N} |\psi_{in}\rangle_b. \end{aligned} \quad (\text{S88})$$

The dummy-mode vacuum projector can be inserted between  $\hat{U}_{bs}^{(4)}$  and  $\tilde{U}_a$  on the last line because no terms to the right of the projector act on the dummy modes and the dummy modes start in vacuum. To finish commuting the unitary operators to the left, we evaluate the product:

$$\begin{aligned} |0\rangle\langle 0|_a^{\otimes N} \hat{U}_{bs}^{(4)} |0\rangle\langle 0|_v^{\otimes N} &= \prod_{i=1}^N \left[ \left( I_{v;i} \otimes |0\rangle\langle 0|_{a;i} \right) \hat{U}_{bs} [\hat{a}_i, \hat{v}_i; \delta] \left( |0\rangle\langle 0|_{v;i} \otimes I_{a;i} \right) \right] \\ &= \prod_{i=1}^N \left[ \hat{U}_{bs} [\hat{a}_i, \hat{v}_i; 1] \delta^{\hat{a}_i^\dagger \hat{a}_i} |0\rangle\langle 0|_{v;i} \right] \\ &= \hat{U}_{bs}^{(4')} \delta^{\hat{n}_a} |0\rangle\langle 0|_v^{\otimes N}, \end{aligned} \quad (\text{S89})$$

where  $\hat{U}_{bs}^{(4')} = \prod_{i=1}^N \hat{U}_{bs} [\hat{a}_i, \hat{v}_i; 1]$  is a complete swap between the real and dummy optical modes and  $\hat{n}_a = \sum_{i=1}^N \hat{a}_i^\dagger \hat{a}_i$  is the total number of photons in the real optical modes. To find Eq. (S89), we used resolutions of the identity and

transformed the mode operators, as in Eq. (S80). Combining Eqs. (S88)–(S89), the final state of the OM system is

$$|\Psi_f'\rangle_{vab} = \hat{U}_{bs}^{(4')} \tilde{U}_a \hat{U}_{bs}^{(1)} \left[ \prod_{i=1}^N \delta^{(r_i \hat{a}_i + t_i \hat{b}_i)^\dagger (r_i \hat{a}_i + t_i \hat{b}_i)} \right] \left[ \prod_{i=1}^N \frac{1}{\sqrt{\nu_i!}} \left( \sqrt{\eta} \sum_{j=1}^N f_{ij} t_j \hat{b}_j \right)^{\nu_i} \right] |0\rangle_v^{\otimes N} |0\rangle_a^{\otimes N} |\psi_{in}\rangle_b, \quad (\text{S90})$$

commuting  $\delta^{\hat{n}_a}$  through the unitary operators. The norm-squared of this state gives the probability of getting detection pattern  $\{\nu_i\}$  with lossy detectors:

$$\begin{aligned} P'_{\{\nu_i\}}(\{t_i\}) &:= \langle \Psi_f' | \Psi_f' \rangle_{vab} \\ &= \langle 0|_a^{\otimes N} \langle \psi_{in}|_b \left[ \prod_{i=1}^N \frac{1}{\sqrt{\nu_i!}} \left( \sqrt{\eta} \sum_{j=1}^N f_{ij} t_j \hat{b}_j \right)^{\nu_i} \right] \left[ \prod_{i=1}^N \delta^{2(r_i \hat{a}_i + t_i \hat{b}_i)^\dagger (r_i \hat{a}_i + t_i \hat{b}_i)} \right] \\ &\quad \times \left[ \prod_{i=1}^N \frac{1}{\sqrt{\nu_i!}} \left( \sqrt{\eta} \sum_{j=1}^N f_{ij} t_j \hat{b}_j \right)^{\nu_i} \right] |0\rangle_a^{\otimes N} |\psi_{in}\rangle_b. \end{aligned} \quad (\text{S91})$$

The dummy modes have already been eliminated from this expression. To eliminate the real optical modes, we use

$$\delta^{2(r_i \hat{a}_i + t_i \hat{b}_i)^\dagger (r_i \hat{a}_i + t_i \hat{b}_i)} = \exp \left[ 2 \ln(\delta) (r_i \hat{a}_i + t_i \hat{b}_i)^\dagger (r_i \hat{a}_i + t_i \hat{b}_i) \right] = \mathcal{N} \left\{ \exp \left[ -\eta (r_i \hat{a}_i + t_i \hat{b}_i)^\dagger (r_i \hat{a}_i + t_i \hat{b}_i) \right] \right\}, \quad (\text{S92})$$

where  $\mathcal{N}\{\bullet\}$  represents the normal ordering. This follows from the relation  $\exp[s\hat{a}^\dagger \hat{a}] = \mathcal{N}\{\exp[(e^s - 1)\hat{a}^\dagger \hat{a}]\}$  for the generic bosonic operator  $\hat{a}$ , and  $\eta = 1 - \delta^2$ . Combining Eqs. (S91) and (S92), the probability of detection outcome  $\{\nu_i\}$  with optical loss is

$$\begin{aligned} P'_{\{\nu_i\}}(\{t_i\}) &= \langle 0|_a^{\otimes N} \langle \psi_{in}|_b \left[ \prod_{i=1}^N \frac{1}{\sqrt{\nu_i!}} \left( \sqrt{\eta} \sum_{j=1}^N f_{ij} t_j \hat{b}_j \right)^{\nu_i} \right] \left[ \prod_{i=1}^N \mathcal{N} \left\{ \exp \left[ -\eta t_i^2 \hat{b}_i^\dagger \hat{b}_i \right] \right\} \right] \\ &\quad \times \left[ \prod_{i=1}^N \frac{1}{\sqrt{\nu_i!}} \left( \sqrt{\eta} \sum_{j=1}^N f_{ij} t_j \hat{b}_j \right)^{\nu_i} \right] |0\rangle_a^{\otimes N} |\psi_{in}\rangle_b \\ &= \langle \psi_{in}|_b \left[ \prod_{i=1}^N \frac{1}{\sqrt{\nu_i!}} \left( \sum_{j=1}^N f_{ij} \sqrt{\eta} t_j \hat{b}_j \right)^{\nu_i} \right] \left[ \prod_{i=1}^N (1 - \eta t_i^2)^{\hat{b}_i^\dagger \hat{b}_i} \right] \left[ \prod_{i=1}^N \frac{1}{\sqrt{\nu_i!}} \left( \sum_{j=1}^N f_{ij} \sqrt{\eta} t_j \hat{b}_j \right)^{\nu_i} \right] |\psi_{in}\rangle_b \\ &= P_{\{\nu_i\}}(\{\sqrt{\eta} t_i\}), \end{aligned} \quad (\text{S93})$$

showing that the probability of detection pattern  $\{\nu_i\}$  using OM beam-splitting transmission amplitude  $\{t_i\}$  and detectors with efficiency  $\eta$  can be calculated from the detection probability with ideal detectors ( $P_{\{\nu_i\}}(\{t_i\})$ , Eq. (S87)) by rescaling the retrieval probabilities. This result lets us calculate the total heralding probability, used in our Bayesian expression for the heralding fidelity (Eq. (21)).

#### D. “Herald-minus-one” detection probability

Here we show that the probability of a getting an apparently successful GHZ herald including a single detector dark count is  $2p_d n^2 (\eta p_{re})^{n-1} (1 - \eta p_{re})^{n+1}$ . This result is used when calculating the GHZ-state heralding fidelity using Bayes’ theorem (Eq. (21)).

As in Sec. S9 A, we take  $\{s_i\}$  to be the parity bits describing the herald detection pattern. We suppose, without loss of generality, that detector pair  $n$  does not detect a photon, so there are only  $n - 1$  parity bits. This describes a “herald-minus-one” detection pattern because it can be flipped to a successful herald detection pattern by a single dark count on either detector in detector pair  $n$ . The (unnormalized) state of the acoustic modes after a herald-minus-one

detection outcome is

$$\begin{aligned}
|\psi''_{\mathbf{f}}\rangle &= \langle 0|_a^{\otimes 2n} \left( \prod_{i=1}^{n-1} \hat{d}_{[i,s_i]} \right) U_{\text{tot}} |0\rangle_a^{\otimes 2n} \cdot |1\rangle_b^{\otimes 2n} \\
&= \left( \frac{t}{\sqrt{2}} \right)^{n-1} r^{\hat{n}_{\text{ph}}} \prod_{i=1}^{n-1} \left( \hat{b}_{[i,+]} - s_i \hat{b}_{[i+1,-]} \right) |1\rangle_b^{\otimes 2n} \\
&= \left( \frac{t}{\sqrt{2}} \right)^{n-1} r^{n+1} \left[ \sum_{m=0}^{n-1} \left( \prod_{k=m+1}^{n-1} s_k \right) |+\text{L}\rangle^{\otimes m} |11\rangle |-\text{L}\rangle^{\otimes n-1-m} \right].
\end{aligned} \tag{S94}$$

The first and second line are calculated as per Eq. (S78)–(S80). The third line can be proven by induction. The norm of this state is  $n(t^2/2)^{n-1}(r^2)^{n+1}$ . There are  $n$  choices for which detector pair has no detection, and there are  $2^{n-1}$  possible detection patterns for the remaining  $n-1$  detector pairs. Therefore, there are  $n2^{n-1}$  possible herald-minus-one detection patterns. The probability that a herald-minus-one detection outcome is flipped to a herald pattern is  $2p_d$ , where  $p_d$  is the dark-count probability of a single detector.<sup>7</sup> Therefore, the total probability of a getting a GHZ herald by way of a detector dark count is  $2p_d n^2 (\eta p_{\text{re}})^{n-1} (1 - \eta p_{\text{re}})^{n+1}$ , making the identification  $t^2 = 1 - r^2 = p_{\text{re}}$  and using the result from Sec. S9 C to include the detection system efficiency,  $\eta$ .

### E. Heralding simulations

Our expression for the GHZ-state heralding probability, Eq. (S74), and fidelity, (S75), are validated by QuTiP simulations of the circuit shown in Fig. S4 and 7. We use the `mcsolve` function of QuTiP 5.0 [6, 7, 19]. This function allows for monitored (stochastic) and unmonitored (deterministic) collapse operators, like `photocurrent_mesolve` in QuTiP 4.7 (see Sec. S4 E), but it is more computationally efficient. The simulation output is a density matrix, and we calculate the overlap with an ideal Bell state to determine the Bell-state heralding fidelity. We only perform simulations for the target parameter set.

There are four acoustic and four optical modes,  $\hat{b}_{[i,q]}$  and  $\hat{a}_{[i,q]}$ , respectively. The mode indices take the values  $i \in \{1, 2\}$  and  $q \in \{0, 1\}$ . The optomechanical beam-splitting interaction between each acoustic mode and its corresponding optical mode is directly simulated using a time-dependent effective beam-splitting Hamiltonian (Eq. (4)). Simulation details are largely the same as those used in the single-phonon heralding simulation (Sec. S4 E), with differences noted below:

- Acoustic modes start in the single-phonon state
- Beam-splitting drive peak powers are  $P_r = 0.1, 0.2, \dots, 0.5$  mW
- Beam-splitting drive duration is  $\tau = 1.18$  ns, with pulse center and simulation duration derived from this
- Monitored collapse operators (detected modes) are

$$\begin{aligned}
\hat{a}'_{[1,0]} &= \sqrt{\eta_d \kappa^{\text{ex}}} (\hat{a}_{[1,0]} + \hat{a}_{[1,1]} + \hat{a}_{[2,0]} - \hat{a}_{[2,1]})/2, & \hat{a}'_{[1,1]} &= \sqrt{\eta_d \kappa^{\text{ex}}} (\hat{a}_{[1,0]} - \hat{a}_{[1,1]} + \hat{a}_{[2,0]} + \hat{a}_{[2,1]})/2, \\
\hat{a}'_{[2,0]} &= \sqrt{\eta_d \kappa^{\text{ex}}} (\hat{a}_{[1,0]} - \hat{a}_{[1,1]} - \hat{a}_{[2,0]} - \hat{a}_{[2,1]})/2, & \hat{a}'_{[2,1]} &= \sqrt{\eta_d \kappa^{\text{ex}}} (\hat{a}_{[1,0]} + \hat{a}_{[1,1]} - \hat{a}_{[2,0]} + \hat{a}_{[2,1]})/2
\end{aligned}$$

All trajectories where two detectors each detected one photon were considered heralds. This includes more heralds than our analytical result and allows for cases where Bell states are prepared in a different dual-rail basis than the predefined basis. This choice decreases simulation uncertainty, increases the heralding probability by  $3/2$ , and does not affect the heralding fidelity. Dark counts are not included in simulation results as they contribute negligibly at the heralding probabilities simulated.

## S10. ITERATIVE GHZ-STATE PREPARATION IN PHONONIC MEMORIES (BLEEDING)

In Sec. S9, we described the preparation of an  $n$ -GHZ state in a single shot, i.e. without feedback or iteration. In this section, we show how the  $n$ -GHZ state may be prepared iteratively, as described in Sec. III C of the main text. As

<sup>7</sup> We assume that the dark count probability is low enough that  $(1 - p_d)^{n-1} \approx 1$

before, we start with a single phonon in each of  $2n$  modes. The successful herald detection patterns are the same: one detection on each pair  $\{[i, 1], [i + 1, 0]\}$  of detectors. Recall that the qubit labels  $i$  are periodic, so one of the detector pairs is  $\{[n, 1], [1, 0]\}$ . When there is a detection on  $[i, 1]$  or  $[i + 1, 0]$ , we say that mode pairs  $i$  and  $i + 1$  are *fused*. The GHZ state is prepared when every set of neighboring mode pairs has been fused (including mode pairs  $n$  and  $1$ ). The key difference between Sec. S9 and this section is that we do not require all  $n$  detections to occur at the same time. This scheme is adapted from [20]. Differences arise because we assume that the acoustic modes may not be directly beam-split with each other. Instead, acoustic modes must be read out and their optical-mode counterparts interfered.

We now describe the bleeding protocol and quantify the effects of zero or one photon detection. In each round, all mode pairs which have not already been fused to both neighbors are read out, and the optical modes are passed through the beam-splitting network described in Sec. S9.<sup>8</sup> The Kraus operators are determined by propagating the detected photon (if any) and the acoustic identity operator back through the beam splitters and tracing out the optical modes. See Eq. (S78)–(S83) for a similar calculation. If no photons are detected, any phonons that were read out experience no-jump back-action, described by the Kraus operator

$$\hat{\mathbb{K}}^{\text{nj}}(p_{\text{re}}) = \prod_{i \in S_{\text{NF}}} \hat{K}_i^{\text{nj}}(p_{\text{re}}); \quad \hat{K}_i^{\text{nj}}(p_{\text{re}}) = (1 - p_{\text{re}})^{\hat{n}_i/2}, \quad (\text{S95})$$

where  $S_{\text{NF}}$  is the set of mode pairs Not yet Fused to both neighbors and  $\hat{n}_i = \hat{b}_{[i,0]}^\dagger \hat{b}_{[i,0]} + \hat{b}_{[i,1]}^\dagger \hat{b}_{[i,1]}$  is the total number of phonons in mode pair  $i$ . We call  $\hat{K}_i$  a partial Kraus operator.

If a single photon is detected at  $[j, 1]$  or  $[j + 1, 0]$  and mode pairs  $j$  and  $j + 1$  have not already been fused, then mode pairs  $j$  and  $j + 1$  are fused. We call this a success. On the other hand, if mode pairs  $j$  and  $j + 1$  have already been fused, such a detection ruins those mode pairs and any others they were fused to.<sup>9</sup> We call this a failure. In the case of both fusion success and failure, the effect of the detection is described by the fusion Kraus operator:

$$\hat{\mathbb{K}}_{j,j+1}^{\text{F},\pm}(p_{\text{re}}) = \hat{\mathbb{K}}^{\text{nj}}(p_{\text{re}}) \hat{K}_{j,j+1}^{\text{F},\pm}(p_{\text{re}}); \quad \hat{K}_{j,j+1}^{\text{F},\pm}(p_{\text{re}}) = \sqrt{\frac{p_{\text{re}}}{2}} \left( \mathbf{1}_{S_{\text{NF}}}(j) \hat{b}_{[j,+]} \mp \mathbf{1}_{S_{\text{NF}}}(j+1) \hat{b}_{[j+1,-]} \right), \quad (\text{S96})$$

where  $\hat{b}_{[j,\pm]} = \frac{1}{\sqrt{2}}(\hat{b}_{[j,0]} \pm \hat{b}_{[j,1]})$  and  $\mathbf{1}_S(x) = \{1 \text{ if } x \in S; 0 \text{ if } x \notin S\}$  is the indicator function, which accounts for the fact that some mode pairs may not be read out.  $\hat{K}_{j,j+1}^{\text{F},+}$  applies if the single photon is detected in mode  $[j, 1]$  while  $\hat{K}_{j,j+1}^{\text{F},-}$  applies if the single photon is detected in mode  $[j + 1, 0]$  in fusion attempt. Notice that the operator  $\hat{\mathbb{K}}_{\text{GHZ}}^{\{s_i\}}$  in Eq. (S81) is  $\hat{\mathbb{K}}^{\text{nj}}(t^2) \prod_{i=1}^n \hat{K}_{i,i+1}^{\text{F},s_i}(t^2)$ , illustrating the correspondence between the single-shot and bleeding strategies for GHZ state preparation.

Recall that the initial state of the acoustic modes is  $|1\rangle^{\otimes 2n}$  and that the GHZ state is prepared when every set of neighboring mode pairs has been fused. When some, but not all, sets of neighboring mode pairs have been fused, the state of the  $2n$  acoustic modes can be decomposed into a product of “primates” [20]. We call a primate comprising  $m$  mode pairs an  $m$ -primate:

$$|\pi_m^{\lambda,\pm}\rangle_{i\dots j} := \sqrt{\lambda/2} \left( |+_L\rangle_{i\dots j-1}^{\otimes m-1} |11\rangle_j \pm |11\rangle_i |-_L\rangle_{i+1\dots j}^{\otimes m-1} \right) + \sqrt{1-\lambda} \left( |+_L\rangle_i |\zeta\rangle |-_L\rangle_j \right), \quad (\text{S97})$$

which includes mode pairs  $i$  through  $j$ , and has  $m + 1$  excitations.  $|\zeta\rangle$  is a normalized state of the middle  $m - 2$  mode pairs, and its form does not matter.  $\lambda$  encodes how well the outermost mode pairs of the primate are entangled. The 1-primate is  $|\pi_1\rangle_i := |11\rangle_i$ , so the initial state of the acoustic resonators may be written  $|\pi_1\rangle^{\otimes n}$ . Furthermore, the only allowed value of  $\lambda$  for the 2-primate is  $\lambda = 1$ .

A pair of primates is fused when their neighboring outermost mode pairs are fused:

$$|\pi_{m_1}^{\lambda_1}\rangle_{i\dots j} |\pi_{m_2}^{\lambda_2}\rangle_{j+1\dots k} \xrightarrow{\hat{\mathbb{K}}_{j,j+1}^{\text{F},\pm}} |\pi_{m'}^{\lambda'}\rangle_{i\dots k}. \quad (\text{S98})$$

The size of the resulting primate is  $m' = m_1 + m_2$ , and  $\lambda'$  depends on  $\lambda_1$ ,  $\lambda_2$ , and  $p_{\text{re}}$ . The probability that the primates are successfully fused depends on the inputs  $\lambda_1$ ,  $\lambda_2$ ,  $p_{\text{re}}$ , and whether  $m_1$  and  $m_2$  are 1 or greater. Finally,

<sup>8</sup> Depending on which fusions have already been successful, not all optical beam splitters are necessary, but we include them to simplify analysis.

<sup>9</sup> The fact that a single detection can ruin the state is a consequence of our inability to directly beam-split phonons.

an  $n$ -primate may be turned into an  $n$ -GHZ state by fusing its outermost mode pairs to each other:

$$|\pi_n^\lambda\rangle_{i\dots j} \xrightarrow{\hat{\mathbb{K}}_{j,i}^{\text{F},\pm}} |n\text{-GHZ}\rangle. \quad (\text{S99})$$

The probability of success depends on the input  $\lambda$  and on  $p_{\text{re}}$ . Notice the order of the subscripts in  $\hat{\mathbb{K}}_{j,i}^{\text{F},\pm}$  above.

If no more than one photon detection occurs per round, the total probability of a detection outcome can be decomposed into the product of probabilities of outcomes for each mode pair (possible outcomes no-jump or failure) or pair of neighboring mode pairs (possible outcome success). These component probabilities are given in Tab. S1.

We consider a situation with  $n = 6$  mode pairs as an example. Suppose we have thus far fused mode pair 1 with mode pair 2, 2 with 3, and 5 with 6, so we have the state

$$|\psi_2\rangle = |\pi_3^\lambda\rangle_{123} |\pi_1\rangle_4 |\pi_2\rangle_{56} \quad (\text{S100})$$

We still need to fuse mode pair 3 with mode pair 4, 4 with 5, and 6 with 1. Therefore, all mode pairs except mode pair 2 will be read out. The possible outcomes involving one or fewer detections are

| Detection        | Event            | Output                                                                                       | Probability                                                               |
|------------------|------------------|----------------------------------------------------------------------------------------------|---------------------------------------------------------------------------|
| none             | No-jump          | $ \pi_3^{\lambda_{\text{nj}}(\lambda)}\rangle_{123}  \pi_1\rangle_4  \pi_2\rangle_{56}$      | $p_{\text{nj}}^{(m)}(\lambda) p_{\text{nj}}^{(1)} p_{\text{nj}}^{(m)}(1)$ |
| [3, 1] or [4, 0] | Fuse 3 and 4     | $ \pi_4^{\lambda^{(1m)}(\lambda)}\rangle_{1234}  \pi_2\rangle_{56}$                          | $p_{\text{S}}^{(1m)}(\lambda) p_{\text{nj}}^{(m)}(1)$                     |
| [4, 1] or [5, 0] | Fuse 4 and 5     | $ \pi_3^{\lambda_{\text{nj}}(\lambda)}\rangle_{123}  \pi_3^{\lambda^{(1m)}(1)}\rangle_{456}$ | $p_{\text{nj}}^{(m)}(\lambda) p_{\text{S}}^{(1m)}(1)$                     |
| [6, 1] or [1, 0] | Fuse 6 and 1     | $ \pi_1\rangle_4  \pi_5^{\lambda^{(nm)}(\lambda,1)}\rangle_{56123}$                          | $p_{\text{nj}}^{(1)} p_{\text{S}}^{(nm)}(\lambda, 1)$                     |
| [1, 1] or [3, 0] | Ruin 1, 2, and 3 | $ \beta_3\rangle_{123}  \pi_1\rangle_4  \pi_2\rangle_{56}$                                   | $p_{\text{F}}^{(m)}(\lambda) p_{\text{nj}}^{(1)} p_{\text{nj}}^{(m)}(1)$  |
| [5, 1] or [6, 0] | Ruin 5 and 6     | $ \pi_3^{\lambda_{\text{nj}}(\lambda)}\rangle_{123}  \pi_1\rangle_4  \beta_2\rangle_{56}$    | $p_{\text{nj}}^{(m)}(\lambda) p_{\text{nj}}^{(1)} p_{\text{F}}^{(m)}(1)$  |

Refer to Tab. S1 for definitions of probabilities and updated  $\lambda$ s.

### A. Bell state in 2 rounds

In Sec. IIIC, we stated that we can boost the probability of preparing a Bell state to 18.3% when allowing up to two iterations, compared to from  $1/8 = 12.5\%$  in a single shot, neglecting detection imperfections. This result is found by modeling the bleeding strategy as a finite Markov process, see Fig. S7.

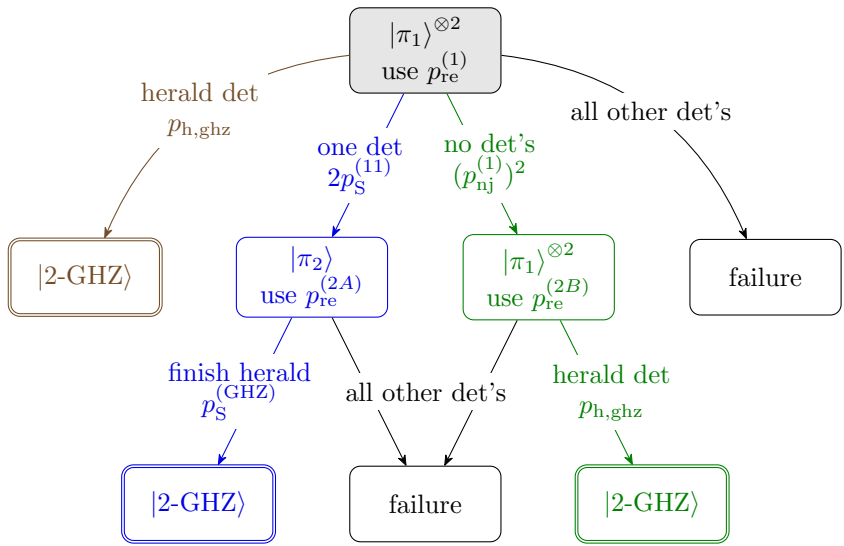

FIG. S7. **Preparing a Bell state in up to two rounds.** The initial state of the acoustic modes is  $|1111\rangle = |\pi_1\rangle^{\otimes 2}$ . After running the Bell-state preparation circuit with retrieval probability  $p_{\text{re}}^{(1)}$ , there are four types of outcomes. The arrows are labeled by the detection (det) pattern and the probability of that detection pattern occurring, and the resulting state is boxed. If there are no detections or there is one detection, we apply the Bell-state preparation circuit to the acoustic modes again, using a different retrieval probability depending on the previous round's outcome. See Eq. (S101) and below for definitions of probabilities, which are color-coded to correspond to the paths of the tree.

The total heralding probability is found by summing the probabilities of the three paths to create a Bell state in

| Input                                                                         | Detection                | Event   | Kraus Operator                                                                         | Output                                                                                                                                                                | Probability                                                                                                   |
|-------------------------------------------------------------------------------|--------------------------|---------|----------------------------------------------------------------------------------------|-----------------------------------------------------------------------------------------------------------------------------------------------------------------------|---------------------------------------------------------------------------------------------------------------|
| $ \pi_1\rangle_i$                                                             | none                     | No-jump | $\hat{\mathbb{K}}^{\text{nj}}$                                                         | unchanged                                                                                                                                                             | $p_{\text{nj}}^{(1)} = R^2$                                                                                   |
| $ \pi_m^\lambda\rangle_{i\dots j}$                                            | none                     | No-jump | $\hat{\mathbb{K}}^{\text{nj}}$                                                         | $ \pi_m^{\lambda_{\text{nj}}}\rangle_{i\dots j}$<br>$\lambda_{\text{nj}}(\lambda) = \frac{R\lambda}{1-\lambda T}$                                                     | $p_{\text{nj}}^{(m)}(\lambda) = R^2(1 - \lambda T)$                                                           |
| $ \pi_m^\lambda\rangle_{i\dots j}$                                            | $[i, 1]$ or $[j, 0]$     | Failure | $\hat{\mathbb{K}}_{i,i+1}^{\text{F},\pm}$ or $\hat{\mathbb{K}}_{j-1,j}^{\text{F},\pm}$ | $ \beta_m\rangle_{i\dots j}$                                                                                                                                          | $p_{\text{F}}^{(m)}(\lambda) = 2RT(1 - \lambda T)$                                                            |
| $ \pi_n^\lambda\rangle_{i\dots j}$                                            | $[j, 1]$ or $[i, 0]$     | Success | $\hat{\mathbb{K}}_{j,i}^{\text{F},\pm}$                                                | $ n\text{-GHZ}\rangle$                                                                                                                                                | $p_{\text{S}}^{(\text{GHZ})}(\lambda) = \lambda R^2 T$                                                        |
| $ \pi_1\rangle_i  \pi_1\rangle_{i+1}$                                         | $[i, 1]$ or $[i + 1, 0]$ | Success | $\hat{\mathbb{K}}_{i,i+1}^{\text{F},\pm}$                                              | $ \pi_2\rangle_{i,i+1}$                                                                                                                                               | $p_{\text{S}}^{(11)} = 2R^3 T$                                                                                |
| $ \pi_1\rangle_i  \pi_m^\lambda\rangle_{i+1\dots j}$                          | $[i, 1]$ or $[i + 1, 0]$ | Success | $\hat{\mathbb{K}}_{i,i+1}^{\text{F},\pm}$                                              | $ \pi_{m+1}^{\lambda^{(1m)}}\rangle_{i\dots j}$<br>$\lambda^{(1m)}(\lambda) = \frac{2R\lambda}{2+\lambda-3\lambda T}$                                                 | $p_{\text{S}}^{(1m)}(\lambda) = \frac{1}{2}R^3 T(2 + \lambda - 3\lambda T)$                                   |
| $ \pi_n^{\lambda_1}\rangle_{i\dots j}  \pi_m^{\lambda_2}\rangle_{j+1\dots k}$ | $[j, 1]$ or $[j + 1, 0]$ | Success | $\hat{\mathbb{K}}_{j,j+1}^{\text{F},\pm}$                                              | $ \pi_{n+m}^{\lambda^{(nm)}}\rangle_{i\dots k}$<br>$\lambda^{(nm)}(\lambda_1, \lambda_2) = \frac{R\lambda_1\lambda_2}{\lambda_1 + \lambda_2 - 2\lambda_1\lambda_2 T}$ | $p_{\text{S}}^{(nm)}(\lambda_1, \lambda_2) = \frac{1}{2}R^4 T(\lambda_1 + \lambda_2 - 2\lambda_1\lambda_2 T)$ |

TABLE S1. Probabilities and outputs of all events involving zero or one photon detection when attempting to fuse primates. Expressions for Kraus operators can be found in Eqs. (S95) and (S96). Assume  $n, m > 1$  unless otherwise specified.  $|\beta_m\rangle$  is a state of  $m$  mode pairs which must be reset. We use  $T = p_{\text{re}}$  and  $R = 1 - T$  for compactness.

up to 2 rounds of bleeding:

$$P_2(p_{\text{re}}^{(1)}, p_{\text{re}}^{(2A)}, p_{\text{re}}^{(2B)}) = \underbrace{p_{\text{h,ghz}}(p_{\text{re}}^{(1)})}_{p_{\text{h}}^{(02)}} + \underbrace{2p_{\text{S}}^{(11)}(p_{\text{re}}^{(1)}) \cdot p_{\text{S}}^{(\text{GHZ})}(1, p_{\text{re}}^{(2A)})}_{p_{\text{h}}^{(012)}} + \underbrace{\left(p_{\text{nj}}^{(1)}(p_{\text{re}}^{(1)})\right)^2 \cdot p_{\text{h,ghz}}(p_{\text{re}}^{(2B)})}_{p_{\text{h}}^{(002)}}, \quad (\text{S101})$$

where  $p_{\text{h,ghz}}(p_{\text{re}})$  is the single-shot success probability (Eq. (S74)) with  $n = 2$ ,  $\eta = 1$ , and  $p_{\text{d}} = 0$ . The bleeding-type success probabilities,  $p_{\text{S}}^{(11)}(T)$  and  $p_{\text{S}}^{(\text{GHZ})}(\lambda, T)$ , can be found in Tab. S1. We numerically maximize  $P_2$  over  $p_{\text{re}}^{(1)}$ ,  $p_{\text{re}}^{(2A)}$ , and  $p_{\text{re}}^{(2B)}$ . The maximum 2-round heralding probability is  $P_2 = 0.183 = 0.109 + 0.055 + 0.019$ , which is achieved when  $p_{\text{re}}^{(1)} = 0.37$ ,  $p_{\text{re}}^{(2A)} = 1/3$ , and  $p_{\text{re}}^{(2B)} = 1/2$ .

### 1. Detection inefficiency and heralding fidelity

We calculate the heralding fidelity for Bell state preparation in up to two rounds, accounting for optical loss. We take  $\eta = \eta_{\text{ex}}\eta_{\text{d}} = 0.999 \times 0.98$ . The effect of detector dark counts is negligible. The heralding fidelity for each path shown in Fig. S7 is equivalent to the single-shot heralding fidelity,  $F_{\text{h,ghz}}$  (Eq. (S75)) using the effective cumulative retrieval probability,  $p_{\text{re}}^{\text{eff}} = 1 - \prod_{k=1}^M (1 - p_{\text{re}}^{(k)})$  (Eq. (27)). Using the optimal retrieval probabilities found above, the heralding fidelities associated with each path to a Bell state are:  $F_{\text{h}}^{(02)} = 0.976$  when heralding success in the first round;  $F_{\text{h}}^{(012)} = 0.944$  when there is one detection in the first round and the herald is completed in the second round; and  $F_{\text{h}}^{(002)} = 0.914$  when there are no detections in the first round and a full herald detection pattern in the second round.

The heralding probability for preparing a Bell state in up to two rounds of bleeding is slightly changed by the inclusion of detection inefficiency. The bleeding rounds are not independent events. Therefore, we cannot make the simple  $p_{\text{re}} \rightarrow \eta p_{\text{re}}$  substitution as we do to find the single-shot heralding probabilities with loss (Sec. S9C). The heralding probabilities for each path, including optical loss, are

$$p_{\text{h}}^{(02)} = 2 \left(1 - \eta p_{\text{re}}^{(1)}\right)^2 \left(\eta p_{\text{re}}^{(1)}\right)^2 \quad (\text{S102})$$

$$p_{\text{h}}^{(012)} = 4 \left(1 - p_{\text{re}}^{(1)}\right) \left(1 - \eta p_{\text{re}}^{\text{eff},(2A)}\right)^2 \left(\eta p_{\text{re}}^{(1)}\right) \left(\eta p_{\text{re}}^{(2A)}\right) \quad (\text{S103})$$

$$p_{\text{h}}^{(002)} = 2 \left(1 - p_{\text{re}}^{(1)}\right)^2 \left(1 - \eta p_{\text{re}}^{\text{eff},(2B)}\right)^2 \left(\eta p_{\text{re}}^{(2B)}\right)^2 \quad (\text{S104})$$

which reduce to the expressions in Eq. (S101) when  $\eta \rightarrow 1$ . Using the optimal retrieval probabilities found above and  $\eta = 0.979$ , the total heralding probability is  $P_2 = 18.3\% = 0.107 + 0.055 + 0.020$  when accounting for loss, largely unchanged from its value in the ideal case. Similarly, the single-shot heralding probability is 12.5% when including optical loss and taking  $p_{\text{re}} = 1/2$ . The average heralding fidelity when preparing a Bell state in up to two rounds of bleeding is

$$F_2 = \frac{1}{P_2} \left( p_{\text{h}}^{(02)} F_{\text{h}}^{(02)} + p_{\text{h}}^{(012)} F_{\text{h}}^{(012)} + p_{\text{h}}^{(002)} F_{\text{h}}^{(002)} \right) = 0.959. \quad (\text{S105})$$

The heralding fidelity in the single-shot case differs by only  $10^{-4}$  from this. Thus, the bleeding strategy can improve the heralding probability without affecting the heralding fidelity.

## B. Asymptotic success probabilities

In this section, we provide the details for our results in Sec. III C 2, of the asymptotic success probability for building an  $n$ -GHZ state. The asymptotic limit takes the retrieval probability/initial beam splitter transmissivity,  $T \rightarrow 0$  and the number of retrieval attempts  $\rightarrow \infty$ . In this limit, we may neglect no-jump backaction and the possibility of more than one photon being retrieved/detected.

The initial state of the acoustic modes is  $|\psi_{\text{in}}\rangle = |\pi_1\rangle^{\otimes n}$  and the final state is  $|n\text{-GHZ}\rangle$ . The intermediate states of the acoustic modes, after  $0 \leq k < n$  successful fusions, may be decomposed into a product of primates,  $|\psi_k\rangle = |\pi_{m_1}^{\lambda_1}\rangle \dots |\pi_{m_{n-k}}^{\lambda_{n-k}}\rangle$ , where  $m_i$  is the size of each primate ( $\sum_{\ell} m_{\ell} = n$ ) and  $\lambda$  is its quality (see Eq. (S97)). Starting

from state  $|\psi_k\rangle$ , the asymptotic probability of neighboring primates  $|\pi_{m_i}^{\lambda_i}\rangle$  and  $|\pi_{m_j}^{\lambda_j}\rangle$  fusing into  $|\pi_{m_i+m_j}^{\lambda'}\rangle$  is

$$p_{S,\text{asy}}^{(m_i, m_j)}(\lambda_i, \lambda_j) = \lim_{T \rightarrow 0} \frac{p_S^{(m_i, m_j)}(\lambda_i, \lambda_j)}{1 - p_{\text{nj}}^{(\text{tot})}}, \quad (\text{S106})$$

where  $p_{\text{nj}}^{(\text{tot})} = \prod p_{\text{nj}}^{(m_\ell)}(\lambda_\ell)$  is the total no-jump probability for the starting state and  $\lambda' = \lambda^{(m_i, m_j)}(\lambda_i, \lambda_j)$  is the quality of the resulting primate (see Tab. S1). After  $n - 1$  fusions, the state of the acoustic modes is  $|\pi_n^\lambda\rangle$ , and the asymptotic probability of it being fused into the  $n$ -GHZ state is

$$p_{S,\text{asy}}^{(\text{GHZ})}(\lambda_i, \lambda_j) = \lim_{T \rightarrow 0} \frac{p_S^{(\text{GHZ})}(\lambda)}{1 - p_{\text{nj}}^{(n)}(\lambda)}. \quad (\text{S107})$$

We now describe the algorithm, which we implemented in Mathematica, for calculating the asymptotic success probabilities. An intermediate state's decomposition into primates is represented by two lists  $(\vec{m}, \vec{\lambda})$ , where  $\vec{m}$  are the sizes of the primates and  $\vec{\lambda}$  are the  $\lambda$ s for each primate ( $\lambda$  is meaningless for  $m = 1$  and must be 1 for  $m = 2$ ). For example, the state (S100) is represented by  $\vec{m} = [3, 1, 2]$  and  $\vec{\lambda} = [\lambda, 1, 1]$ . Two states are considered equivalent if they are related by rotation or reflection of these lists:  $([m_1, m_2, m_3], [\lambda_1, \lambda_2, \lambda_3]) \Leftrightarrow ([m_2, m_3, m_1], [\lambda_2, \lambda_3, \lambda_1]) \Leftrightarrow ([m_3, m_2, m_1], [\lambda_3, \lambda_2, \lambda_1])$  but  $([m_1, m_2, m_3, m_4], [\lambda_1, \lambda_2, \lambda_3, \lambda_4]) \not\Leftrightarrow ([m_1, m_2, m_4, m_3], [\lambda_1, \lambda_2, \lambda_4, \lambda_3])$ . We iteratively calculate the cumulative probability to reach each non-equivalent intermediate state, and store it as  $(p, \vec{m}, \vec{\lambda})$ , where  $p$  is the cumulative probability to have reached this state. See Fig. S8 for a visual representation of this calculation for  $n = 4$ . Results are presented in Tab. S2.

**function** ASYMPTOTICSUCCESSPROB( $n$ )

```

oldstates  $\leftarrow \{(1, [1, \dots, 1], [1, \dots, 1]), \}$   $\triangleright$  Initial state, represented as  $(p, \vec{m}, \vec{\lambda})$ . Lengths  $|\vec{m}| = |\vec{\lambda}| = n$ 
for  $k = 1, \dots, n - 1$  do  $\triangleright n$  fusions are required. The final one is calculated after the loop
    newstates  $\leftarrow \{\}$   $\triangleright$  Re-initialize
    for all state  $\in$  oldstates do  $\triangleright$  Consider each "starting" state separately
         $(p, \vec{m}, \vec{\lambda}) \leftarrow$  state  $\triangleright$  Unpack state
        for  $i = 1, \dots, |\vec{m}|$  do  $\triangleright$  Loop through the primates that make up the state
             $j \leftarrow i \% |\vec{m}| + 1$   $\triangleright$  Each primate can fuse to the one next to it, wrapping around at the end
             $p_S \leftarrow p_{S,\text{asy}}^{(m_i, m_j)}(\lambda_i, \lambda_j)$   $\triangleright$  Eq. (S106)
             $\vec{m}_{\text{new}} \leftarrow \vec{m}$ , replacing  $m_i$  and  $m_j$  with  $m_i + m_j$ 
             $\vec{\lambda}_{\text{new}} \leftarrow \vec{\lambda}$ , replacing  $\lambda_i$  and  $\lambda_j$  with  $\lambda^{(m_i, m_j)}(\lambda_i, \lambda_j)$   $\triangleright$  Expressions in Tab. S1, let  $T = 0$ 
            Append  $(p \cdot p_S, \vec{m}_{\text{new}}, \vec{\lambda}_{\text{new}})$  to newstates  $\triangleright$  Notice we have multiplied  $p_S$  by the old probability  $p$ 
        Collect equivalent states in newstates and sum their cumulative probabilities together
    oldstates  $\leftarrow$  newstates
state  $\leftarrow$  oldstates[[1]]  $\triangleright$  At this point, there should only be one possible state, which is the  $n$ -primate
 $(p, \vec{m}, \vec{\lambda}) \leftarrow$  state  $\triangleright$  Unpack state
 $p_S \leftarrow p_{S,\text{asy}}^{(\text{GHZ})}(\lambda_1)$   $\triangleright$  Eq. (S107)
return  $p \cdot p_S$ 
```

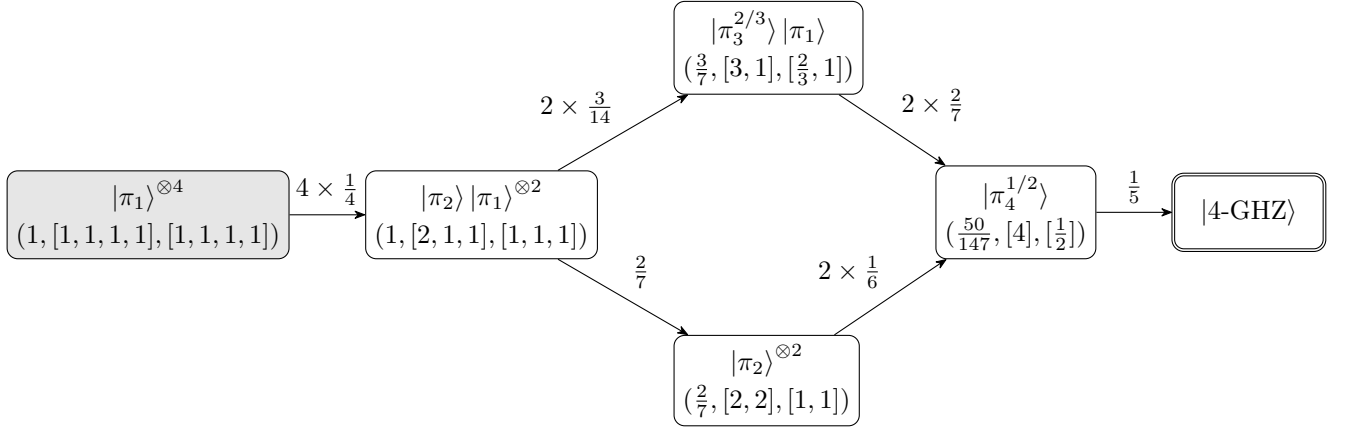

FIG. S8. Asymptotic probabilities for each transition when building 4-GHZ state. Each node represents a class of equivalent states, and is labeled by a representative state for that class. The state is written in conventional quantum notation on the first line and its  $(p, \vec{m}, \vec{\lambda})$  as used in the algorithm on the second line. Integer prefactors in transition probabilities account for the multiple ways to create equivalent states. Final asymptotic probability is  $(4 \times \frac{1}{4}) ((\frac{2}{7})(2 \times \frac{1}{6}) + (2 \times \frac{3}{14})(2 \times \frac{2}{7})) (\frac{1}{5}) = \frac{10}{147}$ .

| $n$ | probability      | $n$ | probability           |
|-----|------------------|-----|-----------------------|
| 2   | $1/3 = 33\%$     | 9   | 0.119%                |
| 3   | $3/20 = 15\%$    | 10  | 0.0527%               |
| 4   | $10/147 = 6.8\%$ | 11  | 0.0233%               |
| 5   | 3.05%            | 12  | 0.0103%               |
| 6   | 1.36%            | 13  | $4.55 \times 10^{-5}$ |
| 7   | 0.607%           | 14  | $2.01 \times 10^{-5}$ |
| 8   | 0.269%           | 15  | $8.87 \times 10^{-6}$ |

TABLE S2. **Asymptotic success probability** for building an  $n$ -GHZ state calculated in Mathematica. Exact probabilities for  $n > 4$  are excluded for legibility.

### C. Rounds-to-success with reset

In this section, we show how we calculated the results in Sec. III C 3 for the number of rounds to prepare the  $n$ -GHZ state with finite retrieval probability.

To calculate the expected number of rounds to successfully prepare an entangled state of 2 or 3 qubits, we must consider the intermediate states on the way to making the full entangled states and the probability of transitioning between each state. For this calculation, we do not consider a “failure” to be an end state. Instead, we define a state “reset” for when a fusion has failed and phononic modes must be reset to the single phonon state. The reset state always returns to the initial state  $|1\rangle^{\otimes 2n} = |\pi_1\rangle^{\otimes n}$  in a set number of rounds. We analytically calculate the expected number of rounds to get from the initial state  $|\pi_1\rangle^{\otimes n}$  to the  $n$ -GHZ state depending on the readout probabilities used at each stage. We validate these analytical values with Monte Carlo simulations of the Markov process. The results in Fig. 10 numerically minimize this analytical expression.

#### 1. 2 qubits

The stochastic process to create a Bell state can be represented by the following diagram:

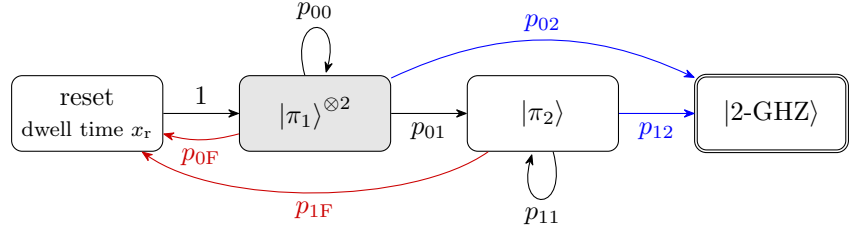

As with the asymptotic probabilities, we consider states which are related by a rotation or reflection of the mode indices to be equivalent:  $|\pi_2\rangle_{12} \Leftrightarrow |\pi_2\rangle_{21}$ . In the process diagram, the subscripts in  $p_{nm}$  indicate the initial and final number of fusions which have cumulatively taken place. The subscript F stands for failure. The probabilities are

$$\begin{aligned}
 p_{00} &= \left(p_{\text{nj}}^{(1)}\right)^2 = (1 - T_0)^4 \\
 p_{01} &= 2p_S^{(11)} = 4T_0(1 - T_0)^3 & p_{11} &= p_{\text{nj}}^{(m)} = (1 - T_1)^3 \\
 p_{02} &= 2T_0^2(1 - T_0)^2 & p_{12} &= p_S^{(\text{GHZ})}(1) = T_1(1 - T_1)^2 \\
 p_{0F} &= 1 - (p_{00} + p_{01} + p_{02}) = T_0^2(2 - T_0)^2 & p_{1F} &= 1 - (p_{11} + p_{12}) = T_1(2 - T_1)
 \end{aligned} \tag{S108}$$

where  $T_0$  is the retrieval probability used when no fusions have been successful yet, and  $T_1$  is the retrieval probability used when one fusion has been successful so far.  $p_{\text{nj}}$  and  $p_S$  refer to values found in Tab. S1, and  $p_{02}$  is the single-shot heralding probability.

To calculate the expected number of rounds,  $\bar{x}^{(2)}$ , until we generate the Bell (or 2-GHZ) state, we need to know how many rounds the system is expected to stay in each state, which we call that state's dwell time, and the branching ratios out of each state. For  $|\pi_1\rangle^{\otimes 2}$  and  $|\pi_2\rangle$ , the dwell times are  $x_0 = 1/(1 - p_{00})$  and  $x_1 = 1/(1 - p_{11})$ . We label the dwell time in the reset state  $x_r = \bar{M}(p_{\text{h,sp}})$ , which is an external parameter controlled by the single-phonon heralding probability (Eq. (16)). The branching ratios are the interstate transition probabilities normalized by  $1 - p_{nn}$ . The total expected number of rounds is calculated from the probability of each path either to the end state (the Bell state) or back to the initial state ( $|\pi_1\rangle^{\otimes 2}$ ). For example, there is a chance  $p_{02}/(1 - p_{00})$  that the first transition the system makes takes you directly to the Bell state, in which case you prepare a Bell state in  $x_0$  rounds, the dwell time of the initial state. On the other hand, there is a chance  $p_{0F}/(1 - p_{00})$  that the first transition the system makes is a failure, in which case you have to start again and just added  $x_0 + x_r$  to the expected number of rounds. All together, the expected number of rounds is found by solving

$$\bar{x}^{(2)} = \frac{p_{02}}{1 - p_{00}}(x_0) + \frac{p_{0F}}{1 - p_{00}}(x_0 + x_r + \bar{x}^{(2)}) + \frac{p_{01}}{1 - p_{00}} \left( \frac{p_{12}}{1 - p_{11}}(x_0 + x_1) + \frac{p_{1F}}{1 - p_{11}}(x_0 + x_1 + x_r + \bar{x}^{(2)}) \right). \tag{S109}$$

## 2. 3 qubits

The stochastic process to generate the 3-GHZ state can be represented by the diagram below:

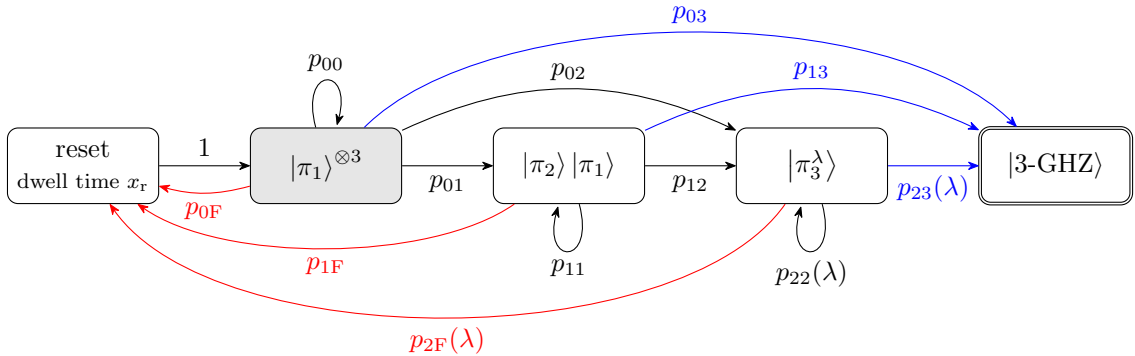

The transition probabilities are

$$\begin{aligned}
p_{00} &= \left(p_{\text{nj}}^{(1)}\right)^3 = (1 - T_0)^6 \\
p_{01} &= 3p_{\text{S}}^{(11)}p_{\text{nj}}^{(1)} = 6T_0(1 - T_0)^5 & p_{11} &= p_{\text{nj}}^{(1)}p_{\text{nj}}^{(m)}(1) = (1 - T_1)^5 \\
p_{02} &= 9T_0^2(1 - T_0)^4 & p_{12} &= 2p_{\text{S}}^{(1m)}(1) = 3T_1(1 - T_1)^4 & p_{22}(\lambda) &= p_{\text{nj}}^{(m)}(\lambda) = (1 - \lambda T_2)(1 - T_2)^2 \\
p_{03} &= 2T_0^3(1 - T_0)^3 & p_{13} &= T_1^2(1 - T_1)^3 & p_{23}(\lambda) &= p_{\text{S}}^{(\text{GHZ})}(\lambda) = \lambda T_2(1 - T_2)^2 \\
p_{0\text{F}} &= 1 - \sum p_{0n} = \mathcal{O}(T_0^2) & p_{1\text{F}} &= 1 - \sum p_{1n} = \mathcal{O}(T_1) & p_{2\text{F}}(\lambda) &= 1 - (p_{22} + p_{23}) = T_2(2 - T_2)
\end{aligned} \tag{S110}$$

As before,  $T_n$  are the retrieval probabilities used when  $n$  fusions have succeeded so far.  $p_{\text{nj}}$  and  $p_{\text{S}}$  refer to values found in Tab. S1, and  $p_{03}$  is the single-shot heralding probability. Other transition probabilities are calculated ad hoc.

Unlike when generating the Bell state, we now have no-jump back-action on the state  $|\pi_3^\lambda\rangle$ . This is simple to deal with in the Monte Carlo simulation, but the analytical computation is complicated by the fact that we no longer have a finite number of possible states. As described in the previous section, we need to know the dwell time and branching ratios for each state. We calculate the expected dwell time,  $\bar{x}_2(\lambda)$  in the state  $|\pi_3^\lambda\rangle$  using the recursive formula

$$\bar{x}_2(\lambda) = \left(1 - p_{\text{nj}}^{(m)}(\lambda)\right) + p_{\text{nj}}^{(m)}(\lambda)\left(1 + \bar{x}_2(\lambda_{\text{nj}}(\lambda))\right).$$

The first term is the probability to leave the state this round multiplied by the dwell time, i.e. 1. The second term is the probability to stay in the state multiplied by the dwell time thus far, 1, plus the expected remaining dwell time taking no-jump back-action into account,  $\bar{x}_2(\lambda_{\text{nj}}(\lambda))$ . Refer to Tab. S1 for  $p_{\text{nj}}$  and  $\lambda_{\text{nj}}$ . The recursion relation is satisfied by

$$\bar{x}_2(\lambda) = \frac{1 - \lambda R_2^2/(1 + R_2 + R_2^2)}{1 - R_2^2},$$

where  $R_2 = 1 - T_2$ . If  $\lambda = 1$  or 0, this simplifies to  $\bar{x}_2(\lambda) = 1/(1 - p_{22}(\lambda))$  because the no-jump back-action has no effect on these initial  $\lambda$ s. For the branching ratio incorporating no-jump back-action, we can calculate the probability that the state  $|\pi_3^\lambda\rangle$  eventually jumps to  $|3\text{-GHZ}\rangle$ ,  $\bar{p}_{23}(\lambda)$ , by the following infinite sum

$$\begin{aligned}
\bar{p}_{23}(\lambda) &= p_{23}(\lambda) + p_{22}(\lambda) \cdot p_{23}(\lambda_{\text{nj}}(\lambda)) + p_{22}(\lambda) \cdot p_{22}(\lambda_{\text{nj}}(\lambda)) \cdot p_{23}(\lambda_{\text{nj}}(\lambda_{\text{nj}}(\lambda))) + \dots \\
&= \sum_{k=1}^{\infty} p_{22}(\lambda, T_2^{(k-1)}) \cdot p_{23}(\lambda_{\text{nj}}(\lambda, T_2^{(k-1)}), T_2) \\
&= \frac{\lambda R_2^2}{1 + R_2 + R_2^2}
\end{aligned}$$

where  $T_2^{(k)} = 1 - (1 - T_2)^k$  is the cumulative retrieval probability, and we used  $p_{22}(\lambda, T) \cdot p_{22}(\lambda_{\text{nj}}(\lambda, T), T') = p_{22}(\lambda, 1 - (1 - T)(1 - T'))$  and  $\lambda_{\text{nj}}(\lambda_{\text{nj}}(\lambda, T), T') = \lambda_{\text{nj}}(\lambda, 1 - (1 - T)(1 - T'))$  to get from the first to the second line. The initial value of  $\lambda$  in  $|\pi_3^\lambda\rangle$  is 2/3, regardless of whether we arrived at this state from  $|\pi_1\rangle|\pi_2\rangle$  or directly from  $|\pi_1\rangle^{\otimes 3}$ . Going forward, we will simply write  $\bar{x}_2 = \bar{x}_2(2/3)$  and  $\bar{p}_{23} = \bar{p}_{23}(2/3)$ . We also let  $\bar{p}_{2\text{F}} = 1 - \bar{p}_{23}$ .

Now, similarly to how we found  $\bar{x}^{(2)}$  (S109), we calculate the expected number of rounds,  $\bar{x}^{(3)}$ , to prepare the 3-GHZ state by the equation

$$\begin{aligned}
\bar{x}^{(3)} &= \frac{p_{03}}{1 - p_{00}}(x_0) + \frac{p_{0\text{F}}}{1 - p_{00}}(x_0 + x_{\text{r}} + \bar{x}^{(3)}) + \frac{p_{02}}{1 - p_{00}} \left[ \bar{p}_{23}(x_0 + \bar{x}_2) + \bar{p}_{2\text{F}}(x_0 + \bar{x}_2 + x_{\text{r}} + \bar{x}^{(3)}) \right] \\
&\quad + \frac{p_{01}}{1 - p_{00}} \left\{ \frac{p_{13}}{1 - p_{11}}(x_0 + x_1) + \frac{p_{1\text{F}}}{1 - p_{11}}(x_0 + x_1 + x_{\text{r}} + \bar{x}^{(3)}) \right. \\
&\quad \left. + \frac{p_{12}}{1 - p_{11}} \left[ \bar{p}_{23}(x_0 + x_1 + \bar{x}_2) + \bar{p}_{2\text{F}}(x_0 + x_1 + \bar{x}_2 + x_{\text{r}} + \bar{x}^{(3)}) \right] \right\}. \tag{S111}
\end{aligned}$$

## S11. OTHER SOURCES OF ENTANGLED OPTICAL PHOTONS

The proposed optomechanical entangled photon source is adapted from all-optical probabilistic entanglement generation [21–23]. As when comparing the optomechanical system to other single photon sources, the advantage of the optomechanical systems as an optical entanglement source lies in the separation of the preparation and retrieval phases, and in the intrinsic time-multiplexing ability of the system. The analysis in Sec. S7 comparing conventional optical multiplexing applies here as well.

Alternatively, probabilistically produced entangled states of optical photons could be stored in quantum memories until needed. See [24] for an overview of working principles and experimental demonstrations of quantum optical memories across many platforms. Optomechanical quantum memories have been demonstrated by [25, 26]. The advantage of our scheme lies in the fact that the entangled state is produced directly in the quantum memory, rather than produced optically and then stored. In this way, it is not dissimilar from the “emissive linear atomic memory protocols” described in [24], proposed by Duan, Lukin, Cirac, and Zoller in 2001 [27]. However, the DLCZ proposal entangles quantum memories in the “single-rail” qubit basis, which is not suitable for fault-tolerant quantum computing. If the quantum optical memory is linear, dual-rail entangled states can only be prepared in the two-step process described in this section—first preparing the single excitations and then entangling them. Our proposal is adaptable to any emissive-type linear quantum optical memory.

Finally, one may directly produce entangled optical photons from quantum emitters, such as quantum dots, single atoms, or defects in diamond. One strategy is to use a single quantum emitter whose successive emissions are entangled [28, 29]. Another strategy is to emit single photons from entangled emitters [30]. For a review of quantum dots as a source of entangled photons, see [31]. Unfortunately, entangled photon sources using from quantum emitters suffer from inadequate extraction efficiency, poor indistinguishability, and decoherence. Furthermore, crystal defects and single atoms are limited in their wavelength availability and engineerability. By contrast, the proposed optomechanical resource can be based in any material platform and engineered to interact with optical photons at any frequency.

- 
- [1] J. E. Sipe and M. J. Steel, A Hamiltonian treatment of stimulated Brillouin scattering in nanoscale integrated waveguides, *New Journal of Physics* **18**, 045004 (2016).
  - [2] C. Wolff, M. J. A. Smith, B. Stiller, and C. G. Poulton, Brillouin scattering—theory and experiment: Tutorial, *JOSA B* **38**, 1243 (2021).
  - [3] M. Aspelmeyer, T. J. Kippenberg, and F. Marquardt, Cavity optomechanics, *Reviews of Modern Physics* **86**, 1391 (2014).
  - [4] H. J. Carmichael, *Statistical Methods in Quantum Optics 1: Master Equations and Fokker-Planck Equations*, Texts and Monographs in Physics (Springer-Verlag, Berlin, Heidelberg, 1999).
  - [5] F. Marquardt, J. P. Chen, A. A. Clerk, and S. M. Girvin, Quantum Theory of Cavity-Assisted Sideband Cooling of Mechanical Motion, *Physical Review Letters* **99**, 093902 (2007).
  - [6] J. R. Johansson, P. D. Nation, and F. Nori, QuTiP: An open-source Python framework for the dynamics of open quantum systems, *Computer Physics Communications* **183**, 1760 (2012).
  - [7] J. R. Johansson, P. D. Nation, and F. Nori, QuTiP 2: A Python framework for the dynamics of open quantum systems, *Computer Physics Communications* **184**, 1234 (2013).
  - [8] K. A. Fischer, R. Trivedi, V. Ramasesh, I. Siddiqi, and J. Vučković, Scattering into one-dimensional waveguides from a coherently-driven quantum-optical system, *Quantum* **2**, 69 (2018).
  - [9] D. Bonneau, G. J. Mendoza, J. L. O’Brien, and M. G. Thompson, Effect of loss on multiplexed single-photon sources, *New Journal of Physics* **17**, 043057 (2015).
  - [10] E. Meyer-Scott, C. Silberhorn, and A. Migdall, Single-photon sources: Approaching the ideal through multiplexing, *Review of Scientific Instruments* **91**, 041101 (2020).
  - [11] F. Kaneda and P. G. Kwiat, High-efficiency single-photon generation via large-scale active time multiplexing, *Science Advances* **5**, eaaw8586 (2019).
  - [12] Z. Hou, J.-F. Tang, C.-J. Huang, Y.-F. Huang, G.-Y. Xiang, C.-F. Li, and G.-C. Guo, Entangled-State Time Multiplexing for Multiphoton Entanglement Generation, *Physical Review Applied* **19**, L011002 (2023).
  - [13] M. Gimeno-Segovia, H. Cable, G. J. Mendoza, P. Shadbolt, J. W. Silverstone, J. Carolan, M. G. Thompson, J. L. O’Brien, and T. Rudolph, Relative multiplexing for minimising switching in linear-optical quantum computing, *New Journal of Physics* **19**, 063013 (2017).
  - [14] W. P. Grice, A. B. U’Ren, and I. A. Walmsley, Eliminating frequency and space-time correlations in multiphoton states, *Physical Review A* **64**, 063815 (2001).
  - [15] I. Aharonovich, D. Englund, and M. Toth, Solid-state single-photon emitters, *Nature Photonics* **10**, 631 (2016).
  - [16] Y. Arakawa and M. J. Holmes, Progress in quantum-dot single photon sources for quantum information technologies: A broad spectrum overview, *Applied Physics Reviews* **7**, 021309 (2020).
  - [17] X. Cao, M. Zopf, and F. Ding, Telecom wavelength single photon sources, *Journal of Semiconductors* **40**, 071901 (2019).
  - [18] E. Bersin, M. Sutula, Y. Q. Huan, A. Suleymanzade, D. R. Assumpcao, Y.-C. Wei, P.-J. Stas, C. M. Knaut, E. N. Knall,

- C. Langrock, N. Sinclair, R. Murphy, R. Riedinger, M. Yeh, C. Xin, S. Bandyopadhyay, D. D. Sukachev, B. Machielse, D. S. Levonian, M. K. Bhaskar, S. Hamilton, H. Park, M. Lončar, M. M. Fejer, P. B. Dixon, D. R. Englund, and M. D. Lukin, Telecom Networking with a Diamond Quantum Memory, [PRX Quantum](#) **5**, 010303 (2024).
- [19] N. Lambert, E. Giguère, P. Menczel, B. Li, P. Hopf, G. Suárez, M. Gali, J. Lishman, R. Gadhvi, R. Agarwal, A. Galicia, N. Shammah, P. Nation, J. R. Johansson, S. Ahmed, S. Cross, A. Pitchford, and F. Nori, [QuTiP 5: The Quantum Toolbox in Python](#) (2024), [arXiv:2412.04705](#).
- [20] S. Bartolucci, P. M. Birchall, M. Gimeno-Segovia, E. Johnston, K. Kieling, M. Pant, T. Rudolph, J. Smith, C. Sparrow, and M. D. Vidrighin, [Creation of Entangled Photonic States Using Linear Optics](#) (2021), [arXiv:2106.13825](#).
- [21] M. Varnava, D. E. Browne, and T. Rudolph, How Good Must Single Photon Sources and Detectors Be for Efficient Linear Optical Quantum Computation?, [Physical Review Letters](#) **100**, 060502 (2008).
- [22] Y. Li, P. C. Humphreys, G. J. Mendoza, and S. C. Benjamin, Resource Costs for Fault-Tolerant Linear Optical Quantum Computing, [Physical Review X](#) **5**, 041007 (2015).
- [23] S. Chen, L.-C. Peng, Y.-P. Guo, X.-M. Gu, X. Ding, R.-Z. Liu, J.-Y. Zhao, X. You, J. Qin, Y.-F. Wang, Y.-M. He, J. J. Renema, Y.-H. Huo, H. Wang, C.-Y. Lu, and J.-W. Pan, Heralded Three-Photon Entanglement from a Single-Photon Source on a Photonic Chip, [Physical Review Letters](#) **132**, 130603 (2024).
- [24] Y. Lei, F. K. Asadi, T. Zhong, A. Kuzmich, C. Simon, and M. Hosseini, Quantum optical memory for entanglement distribution, [Optica](#) **10**, 1511 (2023).
- [25] A. Wallucks, I. Marinković, B. Hensen, R. Stockill, and S. Gröblacher, A quantum memory at telecom wavelengths, [Nature Physics](#) **16**, 772 (2020).
- [26] M. Merklein, B. Stiller, K. Vu, S. J. Madden, and B. J. Eggleton, A chip-integrated coherent photonic-phononic memory, [Nature Communications](#) **8**, 574 (2017).
- [27] L.-M. Duan, M. D. Lukin, J. I. Cirac, and P. Zoller, Long-distance quantum communication with atomic ensembles and linear optics, [Nature](#) **414**, 413 (2001).
- [28] C. Schön, E. Solano, F. Verstraete, J. I. Cirac, and M. M. Wolf, Sequential generation of entangled multiqubit states, [Physical Review Letters](#) **95**, 110503 (2005).
- [29] N. H. Lindner and T. Rudolph, Proposal for Pulsed On-Demand Sources of Photonic Cluster State Strings, [Physical Review Letters](#) **103**, 113602 (2009).
- [30] S. E. Economou, N. Lindner, and T. Rudolph, Optically generated 2-dimensional photonic cluster state from coupled quantum dots, [Physical Review Letters](#) **105**, 093601 (2010).
- [31] D. Huber, M. Reindl, J. Aberl, A. Rastelli, and R. Trotta, Semiconductor quantum dots as an ideal source of polarization-entangled photon pairs on-demand: A review, [Journal of Optics](#) **20**, 073002 (2018).
